# Supplementary material for: RT3D: Achieving Real-Time Execution of 3D Convolutional Neural Networks on Mobile Devices
Source: arXiv:2007.09835 source file (2021-01-03)
Supplement: Supplementary file 1 [file appendix.tex]

\section*{Appendices}

A \emph{demo video} of \projectname is uploaded with Appendices in the Supplementary Material. 
We use the R(2+1)D model on UCF101 dataset with our proposed KGS sparsity scheme and reweighted regularization pruning algorithm as an example.
The inference accuracy of the executed sparse model is $92.0\%$, and pruning rate is 3.2$\times$.
Consistent with the test-bed and evaluation setup in our paper, this \textbf{demo application} runs on a Qualcomm Adreno 650 GPU of a Samsung Galaxy S20 cellphone with the Android 10 Operating System. 
The following figure shows a demo snapshot that consists of three parts: the top part shows a real-time video read from the camera, the middle part shows the inference result ({\tt Billiards}), and the bottom part shows the inference speed in FPS (frames per second).
We use another phone to record this demo video.

This snapshot shows that {\tt Billiards} is recognized from a video displayed on a PC screen. The inference speed is 108 frames/second, corresponding to 148 ms end-to-end inference time for a 16-frame video. 
%This video may contain some wrong recognition between two consecutive 16-frame videos. %\textcolor{blue}{
As the demo also relies on GPU to render User Interface and to decode camera input, the real demo inference speed slightly differs from the one in Table~\ref{tab:performance-report} (in which the FPS is 113).
%}

\begin{figure}[hptb]
  \centering
\includegraphics[width=.25\textwidth]{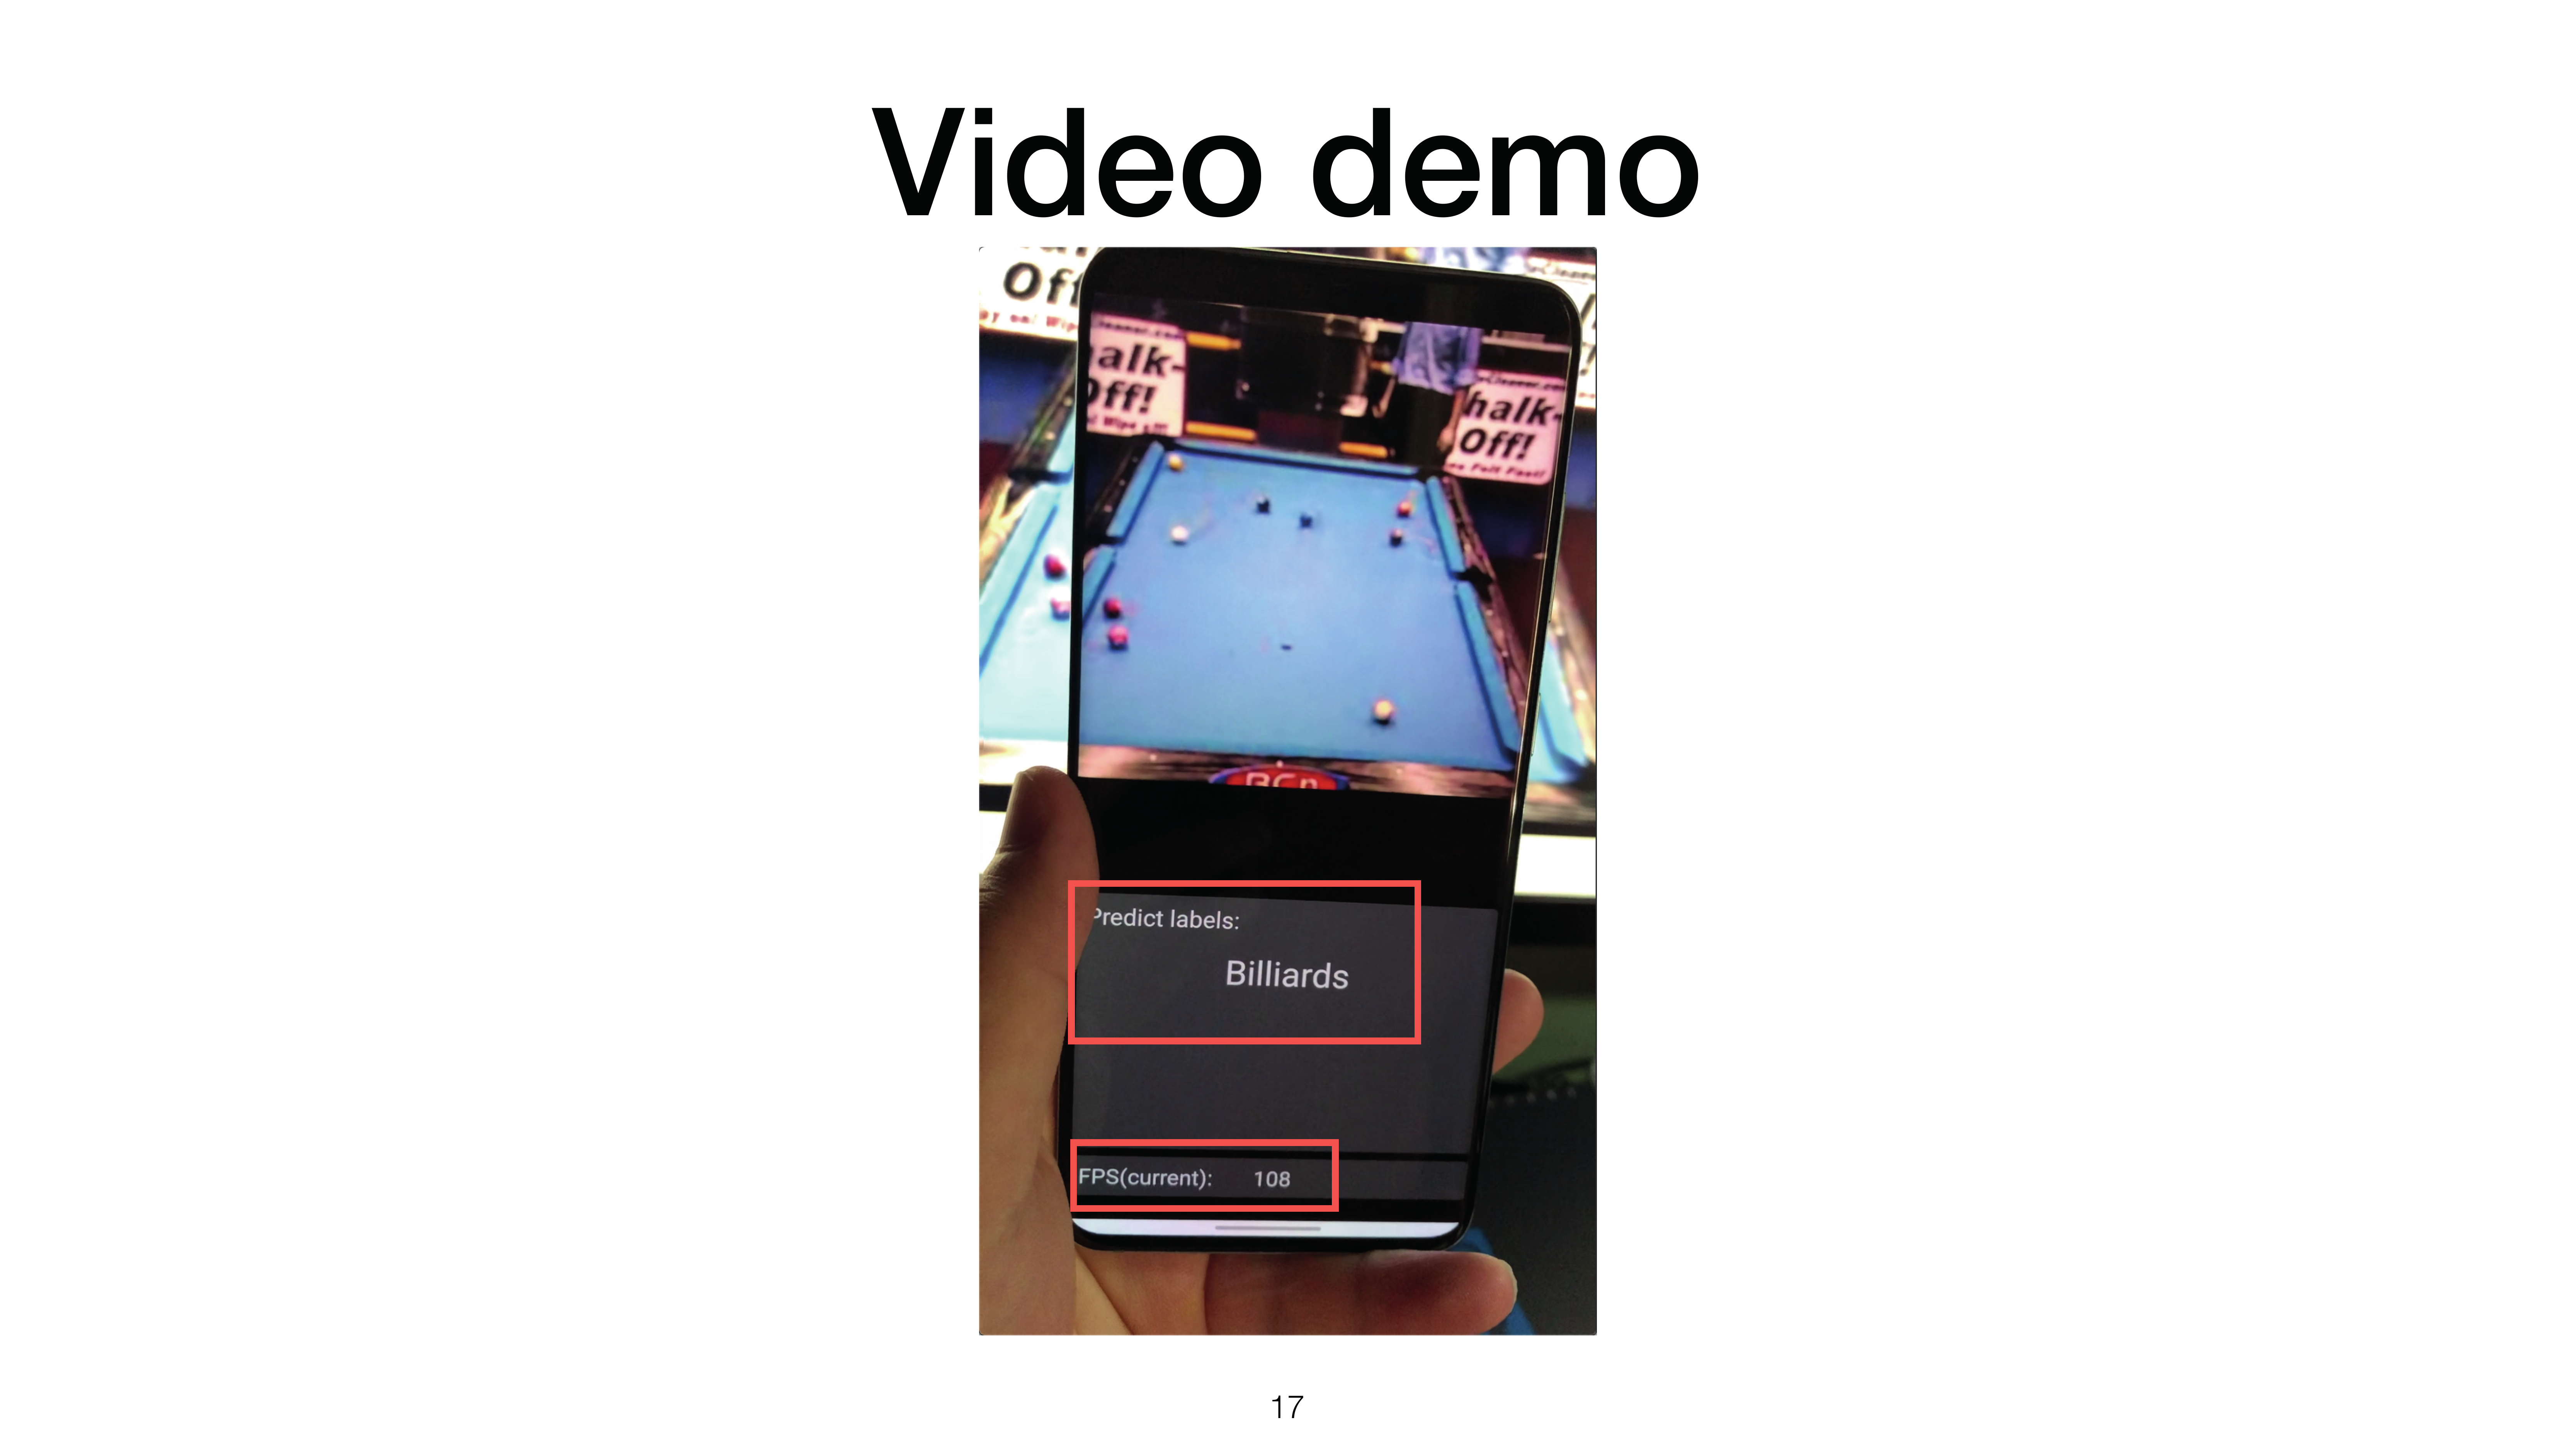}
\end{figure}

\setcounter{section}{0}
\setcounter{figure}{0}
\makeatletter 
\makeatother
\setcounter{table}{0}

\appendix
% \section{Kernel Group Definition}\label{appendix:kernelgroup}

% \begin{figure*}[hptb]
% \centering
% \includegraphics[width=.8\textwidth]{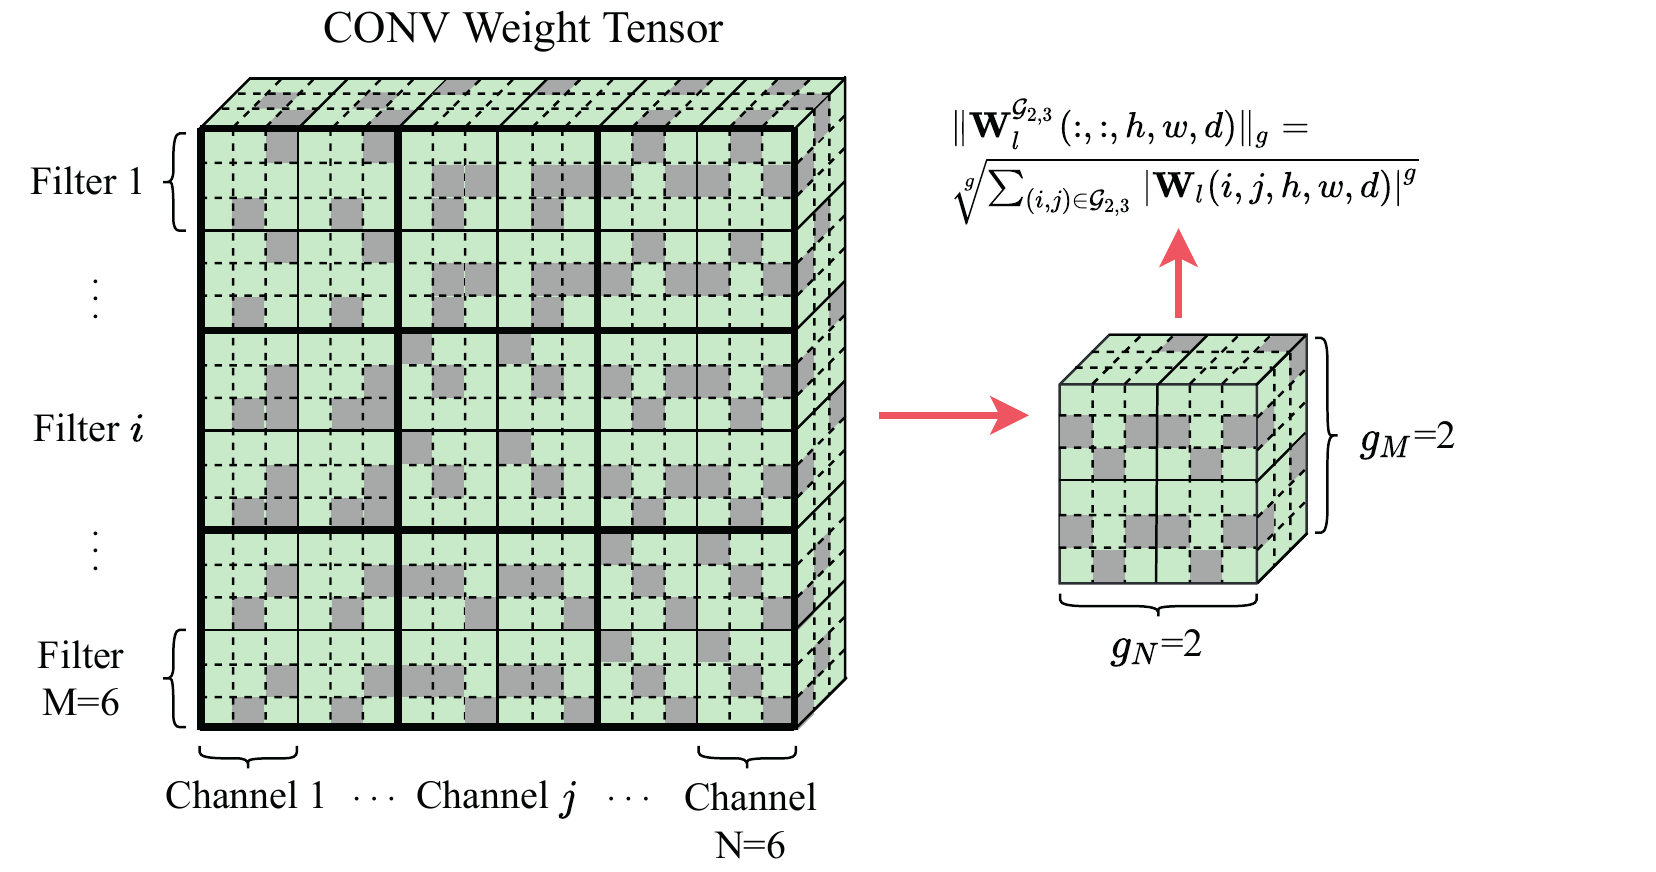}
% \caption {\textbf{An example of kernel groups, each consisting of $g_M\times g_N$ ($2\times 2$) 3D kernels.} Within the same kernel group, kernels are pruned at the same locations (marked by the grey entries). To achieve the same sparsity pattern for kernels in the same group, group lasso is calculated as $\left\|\mathbf{W}_l^{\mathcal{G}_{p,q}}(:,:,h,w,d)\right\|_g=\sqrt[g]{\sum_{(i,j)\in\mathcal{G}_{p,q}}|\mathbf{W}_l(:,:,h,w,d)|^g}$.}
% \label{fig:groupwisesparsity}
% \end{figure*}

\section{Regularization-based Pruning Algorithm for Vanilla Sparsity}\label{appendix:vanilla}

The regularization-based pruning with the Vanilla sparsity scheme can be achieved by 
% \begin{equation}\label{eqn:reg_vanilla}
% \underset{ \{{\mathbf{W}}_{l}\},\{{\mathbf{b}}_{l} \} }{\text{minimize}}\ F \big( \{{\mathbf{W}}_l\}^L_{l=1},\{{\mathbf{b}}_l\}^L_{l=1} \big) + \lambda \sum^L_{l=1}\sum_{p=1}^{P}\sum_{q=1}^{Q} \left\| {\mathbf{W}}_l^{\mathcal{G}_{p,q}} \right\|_g,
% \end{equation}
% where $\left\| \mathbf{W}_l^{\mathcal{G}_{p,q}} \right\|_g = \sqrt[g]{\sum_{(i,j)\in\mathcal{G}_{p,q}} \sum_{h=1}^{K_h}\sum_{w=1}^{K_w}\sum_{d=1}^{K_d} |\mathbf{W}_l(i,j,h,w,d)|^g}$.
\begin{equation}
\label{eqn:reg_vanilla}
% \scalebox{1}{
% \begin{math}
\begin{aligned}
\underset{ \{{\mathbf{W}}_{l}\},\{{\mathbf{b}}_{l} \} }{\text{minimize}}\ & F \big( \{{\mathbf{W}}_l\}^L_{l=1},\{{\mathbf{b}}_l\}^L_{l=1} \big) + \\
& \lambda \sum^L_{l=1}\sum_{p=1}^{P}\sum_{q=1}^{Q} \left\| {\mathbf{W}}_l^{\mathcal{G}_{p,q}} \right\|_g,
% \end{math}
% }
\end{aligned}
\end{equation}
where
\begin{equation}
\nonumber
\left\| \mathbf{W}_l^{\mathcal{G}_{p,q}} \right\|_g = \sqrt[g]{\sum_{(i,j)\in\mathcal{G}_{p,q}} \sum_{h=1}^{K_h}\sum_{w=1}^{K_w}\sum_{d=1}^{K_d} |\mathbf{W}_l(i,j,h,w,d)|^g}.
\end{equation}
This formulation can be generalized to reweighted regularization algorithm as well.

\section{More Pruning Results}\label{appendix:morepruning}

Table~\ref{tab:s3d_ucf} shows the pruning results of the S3D model on UCF101 dataset. Similar to C3D and R(2+1)D results, the reweighted regularization method with KGS sparsity performs the best, achieving 0.4\% accuracy loss with pruning rate of 2.1$\times$.

% S3D results on UCF101
% \begingroup
% \setlength{\tabcolsep}{5.0pt} % Default value: 6pt (cell's horizental space)
% \renewcommand{\arraystretch}{1.0} % Default value: 1 (cell's vertical space)
\begin{table*}[hptb]
\centering
% \small
\begin{tabular}{|c|c|c|c|c|c|c|}
    \hline
    \multirow{2}{*}{Model} & Pruning & Sparsity & Overall FLOPs & Pruning Rate & Base Top-1 & Pruning Top-1 \\
                            & Algorithm & Scheme & after Pruning & of FLOPs & Accuracy & Accuracy \\
    \hline \hline
    \multirow{12}{*}{\makecell{S3D \\ (31MB)}} & \multirow{4}{*}{Heuristic} & Filter & 11.8G & 2.1$\times$ & \multirow{4}{*}{90.6\%} & 86.8\% \\
                             & ~ & Vanilla & 11.8G & 2.1$\times$ & ~ & 87.9\% \\ 
                             & ~ & KGS & 11.8G & 2.1$\times$ & ~ & 88.5\% \\ 
                             & ~ & KGS & 10.3G & 2.4$\times$ & ~ & 87.6\% \\ \cline{2-7}
    
                             & \multirow{4}{*}{Regularization} & Filter & 11.8G & 2.1$\times$ & \multirow{4}{*}{90.6\%} & 87.8\% \\
                             & ~ & Vanilla & 11.8G & 2.1$\times$ & ~ & 89.1\% \\ 
                             & ~ & KGS & 11.8G & 2.1$\times$ & ~ & 89.7\% \\ 
                             & ~ & KGS & 10.3G & 2.4$\times$ & ~ & 88.8\% \\ \cline{2-7}

                             & ~ & Filter & 11.8G & 2.1$\times$ & \multirow{4}{*}{90.6\%} & 88.2\% \\
                             & \textbf{Reweighted} & Vanilla  & 11.8G & 2.1$\times$ & ~ & 89.3\% \\ 
                             & \textbf{Regularization} & \textbf{KGS} & \textbf{11.8G} & \textbf{2.1$\times$} & ~ & \textbf{90.2\%} \\ 
                             & ~ & \textbf{KGS} & \textbf{10.3G} & \textbf{2.4$\times$} & ~ & \textbf{89.1\%} \\ \hline
                             
\end{tabular}
\caption{S3D pruning results on the UCF101 dataset.}
\label{tab:s3d_ucf}
\end{table*}
% \endgroup

% CONV3D results on HMDB51
% \begingroup
% \setlength{\tabcolsep}{5.0pt} % Default value: 6pt (cell's horizental space)
% \renewcommand{\arraystretch}{1.0} % Default value: 1 (cell's vertical space)
\begin{table*}[hp]
\centering
% \small
\begin{tabular}{|c|c|c|c|c|c|c|}
    \hline
    \multirow{2}{*}{Model} & Pruning & Sparsity & Overall FLOPs & Pruning Rate & Base Top-1 & Pruning Top-1 \\
                            & Algorithm & Scheme & after Pruning & of FLOPs & Accuracy & Accuracy \\
    \hline \hline
    % C3D results
    \multirow{6}{*}{\makecell{C3D \\ (299MB)}} & \multirow{3}{*}{Regularization} & Vanilla & 15.2G & 2.6$\times$ & \multirow{3}{*}{53.5\%} & 52.1\% \\
                        & ~ & KGS & 15.2G & 2.6$\times$ & ~ & 53.2\% \\ 
                        & ~ & KGS & 10.8G & 3.6$\times$ & ~ & 52.6\% \\ \cline{2-7}
                            
    ~ & \multirow{3}{*}{\textbf{\makecell{Reweighted \\ Regularization}}} & Vanilla & 15.2G & 2.6$\times$ & \multirow{3}{*}{53.5\%} & 52.8\% \\
                            & ~ & \textbf{KGS} & \textbf{15.2G} & \textbf{2.6}$\times$ & ~ & \textbf{54.0\%} \\ 
                            & ~ & \textbf{KGS} & \textbf{10.8G} & \textbf{3.6}$\times$ & ~ & \textbf{53.7\%} \\ \hline \hline
    % R2+1D results
    \multirow{6}{*}{\makecell{R(2+1)D \\ (120MB)}} & \multirow{3}{*}{Regularization} & Vanilla & 15.9G & 2.6$\times$ & \multirow{3}{*}{71.3\%} & 67.5\% \\
                             & ~ & KGS & 15.9G & 2.6$\times$ & ~ & 67.7\% \\ 
                             & ~ & KGS & 12.7G & 3.2$\times$ & ~ & 67.4\% \\ \cline{2-7}
    
    ~ & \multirow{3}{*}{\textbf{\makecell{Reweighted \\ Regularization}}} & Vanilla & 15.9G & 2.6$\times$ & \multirow{3}{*}{71.3\%} & 68.2\% \\
                             & ~ & \textbf{KGS} & \textbf{15.9G} & \textbf{2.6$\times$} & ~ & \textbf{68.8\%} \\ 
                             & ~ & \textbf{KGS} & \textbf{12.7G} & \textbf{3.2$\times$} & ~ & \textbf{68.3\%} \\ \hline \hline
    
    % S3D results
    \multirow{6}{*}{\makecell{S3D \\ (31MB)}} & \multirow{3}{*}{Regularization} & Vanilla & 11.8G & 2.1$\times$ & \multirow{3}{*}{67.2\%} & 61.9\% \\
                             & ~ & KGS & 11.8G & 2.1$\times$ & ~ & 63.6\% \\ 
                             & ~ & KGS & 10.3G & 2.4$\times$ & ~ & 61.2\% \\ \cline{2-7}

    ~ & \multirow{3}{*}{\textbf{\makecell{Reweighted \\ Regularization}}} & Vanilla & 11.8G & 2.1$\times$ & \multirow{3}{*}{67.2\%} & 63.2\% \\
                             & ~ & \textbf{KGS} & \textbf{11.8G} & \textbf{2.1$\times$} & ~ & \textbf{64.5\%} \\ 
                            & ~ & \textbf{KGS} & \textbf{10.3G} & \textbf{2.4$\times$} & ~ & \textbf{62.0\%} \\ \hline
                             
\end{tabular}
\caption{3D CNN pruning results on the HMDB51 dataset.}
\label{tab:prune_hmdb}
\end{table*}
% \endgroup

The pruning results on HMDB51 dataset with three 3D models, i.e., C3D, R(2+1)D, and S3D are displayed in Table~\ref{tab:prune_hmdb}. Reweighted regularization with KGS sparsity would result in higher accuracy generally. The C3D model with pruning rate of 3.6$\times$ could even outperform the baseline model (without any pruning).

% \clearpage

\section{Mobile Acceleration -- System Design and Compiler Optimization}
\label{sec:appendix-system-design}

\begin{figure*}[hptb]
  \centering
  \includegraphics[width=0.98\textwidth]{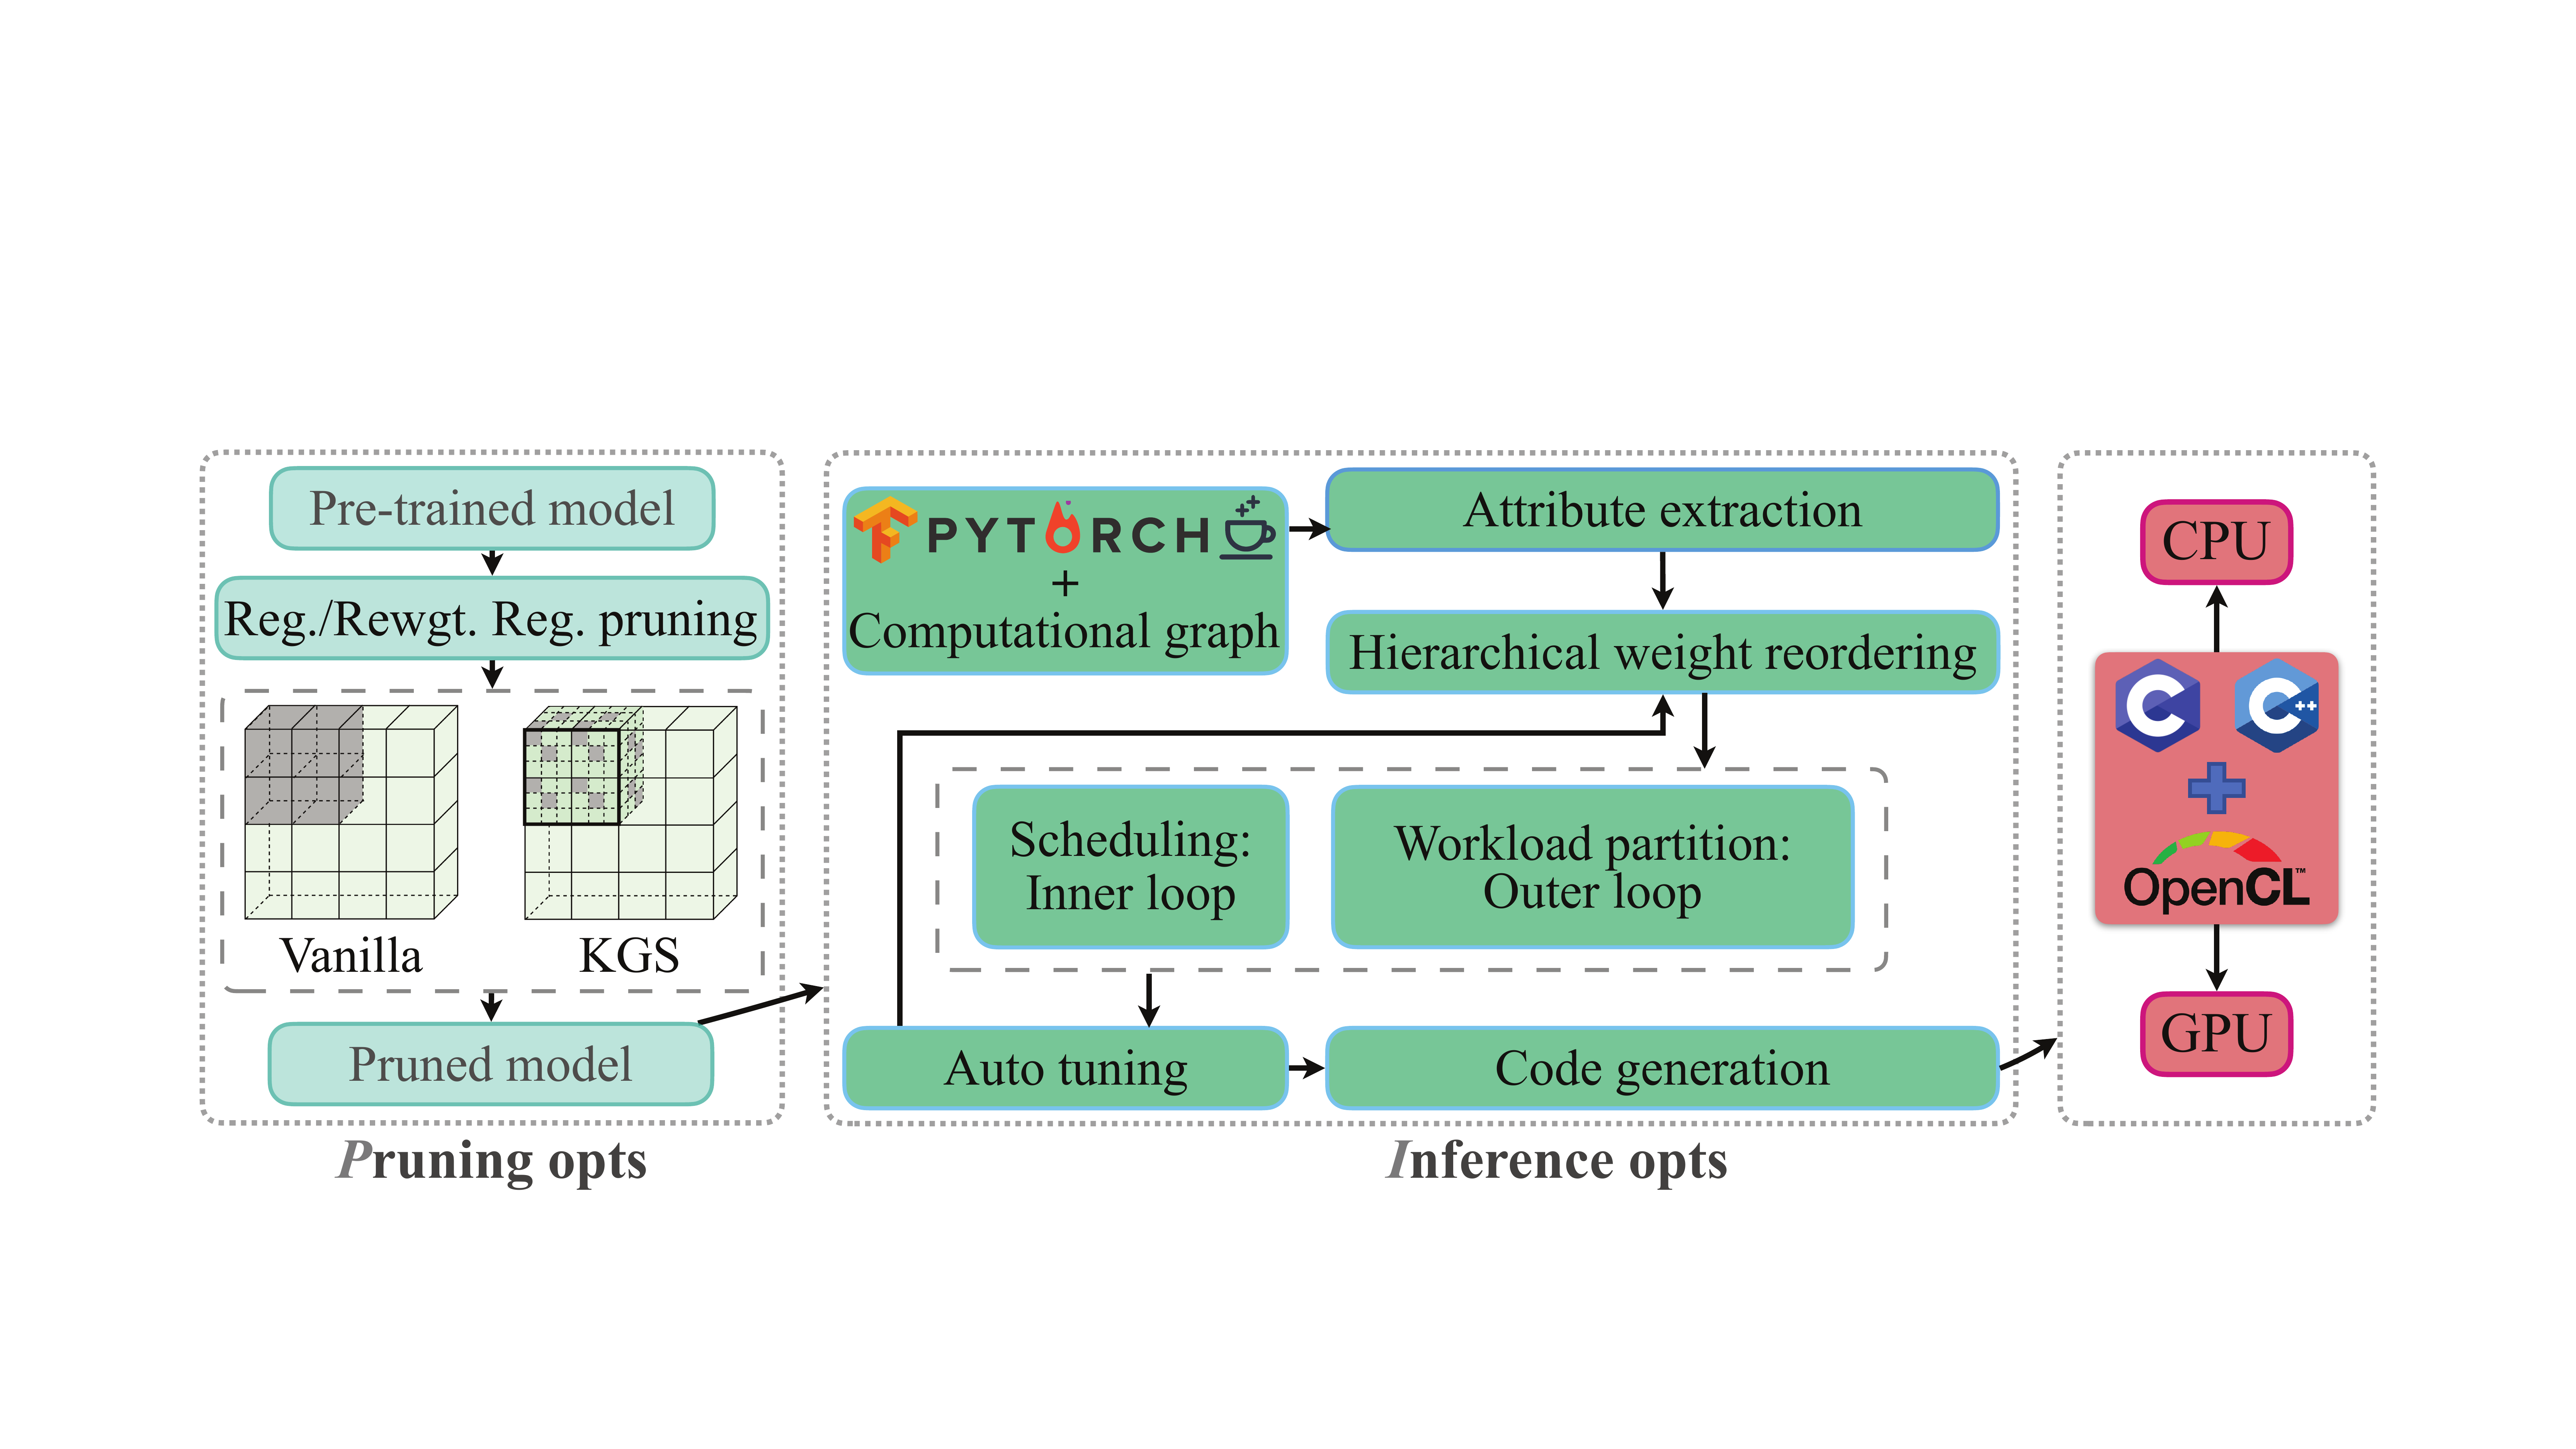}
  \caption{A System Overview of \projectname.}
  \label{fig:overview}
\end{figure*}

%\todo{Match the figure with this text.}

Figure~\ref{fig:overview} shows an overview of \projectname that consists of two main phases: mobile-friendly structured pruning and compiler-optimized inference. As aforementioned, the former phase relies on two structured sparsity schemes, i.e., the vanilla structured sparsity and kernel group structured (KGS) sparsity and their best suited pruning algorithms to generate the compressed model with lossless accuracy.
At the high level, the generated compressed model is represented as a computational graph as TVM~\cite{chen2018tvm} that can support models from varied frameworks like TensorFlow, Pytorch, etc.
Then, the latter phase employs a compiler-based approach to extract the model attributes (particularly the ones related to the pruning), optimize the model storage and computation based on these attributes, and generate the optimized model inference code with optimal configurations that are acquired by auto-tuning. \projectname can generate both optimized CPU (vectorized C++) and GPU (OpenCL) codes.

\paragraph{Hierarchical weight reorder.}
%extreme constraint cache (GPU) friendly
Although our pruning is as SIMD-friendly as possible, it still introduces irregularity to a certain extent. Without further optimization, such irregularity incurs random memory access and thread divergence, and more importantly limits the input data reuse thus still resulting in a large memory footprint. 
To mitigate this problem, \projectname introduces a hierarchical weight reorder (HWR) to reorganize the model weights, and thus reorganize the computation. 

Figure~\ref{fig:fk_reorder} shows an HWR example. HWR performs on each $K_h\times K_w$ section of 3D CONV model with fixed $K_d$. Y-dimension ($K_h$) denotes the filters corresponding to the same input channel while x-dimension ($K_w$) denotes the kernels corresponding to the same output channel. Every conecutive 4 kernels in a filter have identical pruning structures (i.e., $g_N = g_M = 4$) thus only the first one is shown. HWR first reorders the filters, and groups those with high similarity together. Two filters' similarity is defined by the number of nonzero values at identical positions of two filters. For example, the similarity of $Filter_0$ and $Filter_2$ is 3, greater than the similarity 1 between $Filter_0$ and $Filter_1$, so $Filter_0$ and $Filter_2$ are grouped together. HWR next reorders the weights within each filter, with the objective that the weights in different filters corresponding to the same input data are stored in the same position after removing all zeros. Such weight reorders are denoted by red circles. Mobile GPU prefers HWR more than CPU due to its more parallelism and constrained memory/cache capacity.

\begin{figure}[hptb]
  \centering
    \includegraphics[width=0.45\textwidth]{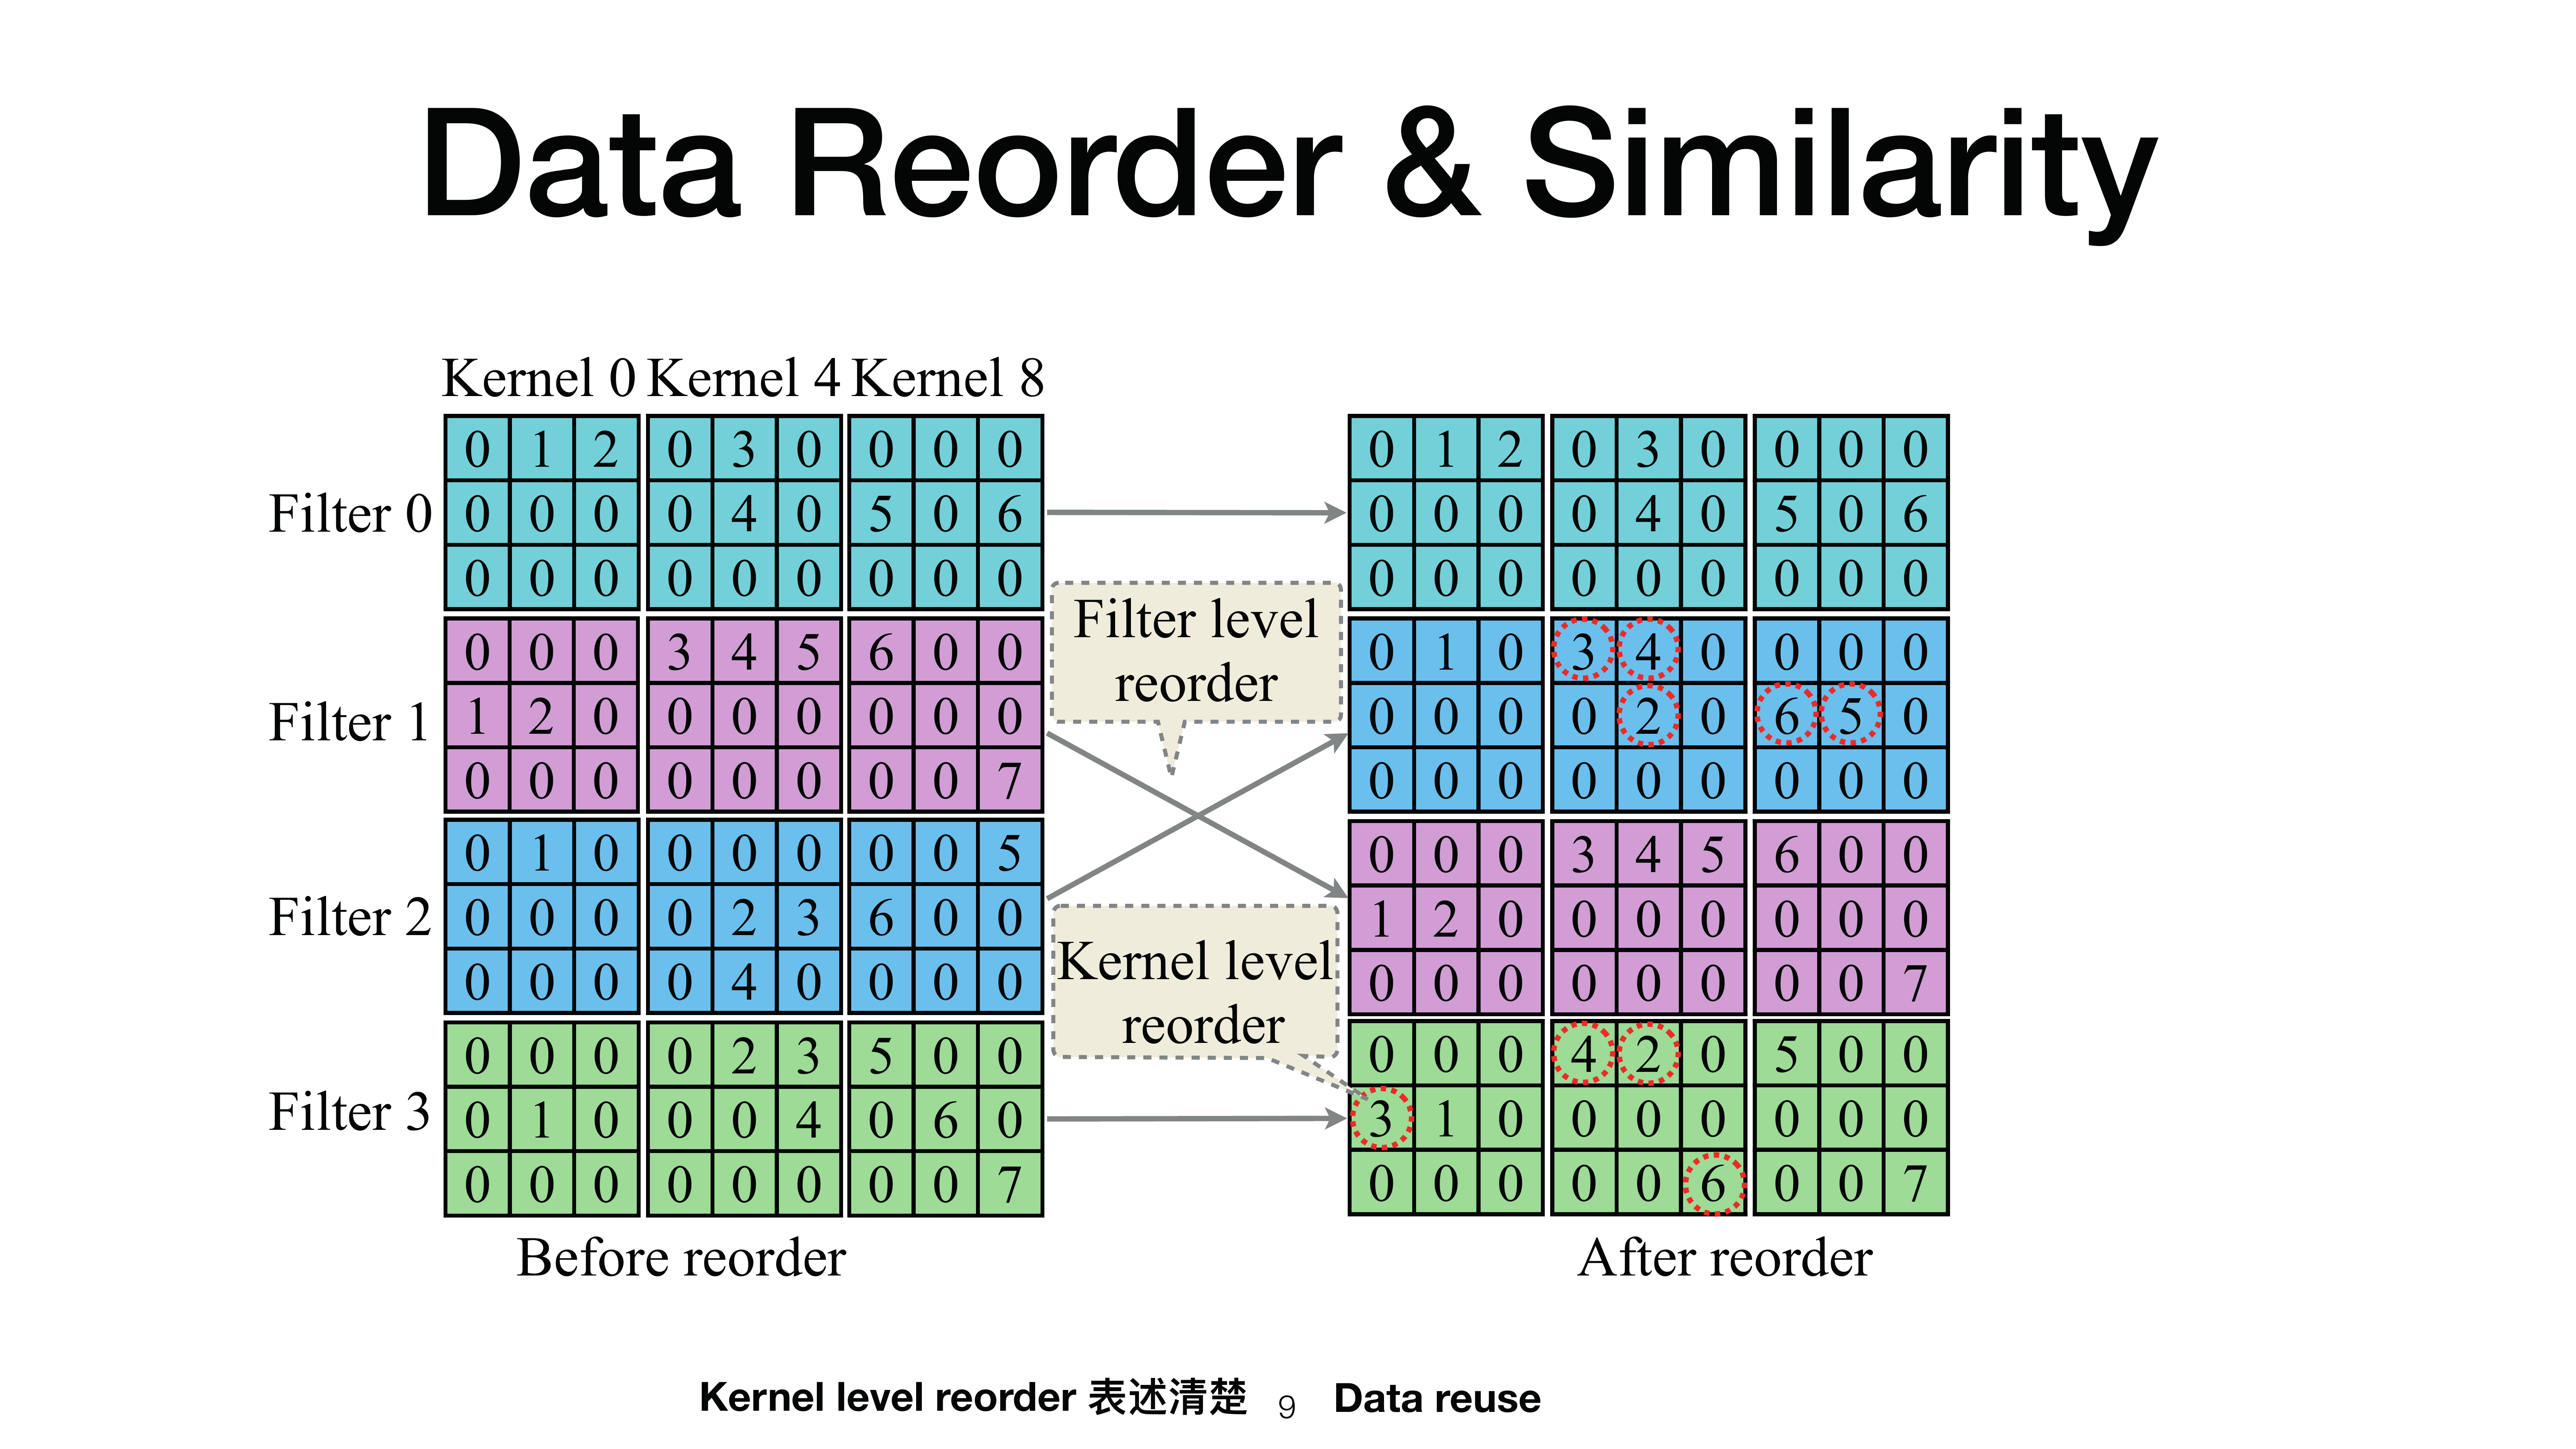}
    \caption{Hierarchical weight reorder.}
    \label{fig:fk_reorder}
\end{figure}

\paragraph{Compact weight storage.} After HWR, \projectname stores nonzero weights in a compact format (CWS) to minimize the model memory footprint. Figure~\ref{fig:compact_storage} shows a simplified example. 
{\em Reorder array} denotes a mapping between the original filter id and the reordered filter position. %, e.g. the filter id 2's index is 1, meaning the original $filter_2$ is reordered to the position 1. 
{\em Offset array} denotes the start position of a certain filter (as Compressed Sparse Row format). %, e.g. 0, 1 and 2 mean the start position of filter0 and filter 1 are 0 and 1, the end position of filter0 and filter 1 are 1 and 2. Generally speaking, for a certain filter x, the start position and length are array[x] and array[x + 1] - array[x].
 {\em Weight array} similarly stores the nonzero weights in a compact 1D array.
{\em Index array} stores the index of each nonzero weight in one byte. Each index has four dimensions, 1 byte per dimension, stored in the order of [$K_d$, $K_h$, $K_w$, $C_i$/4] (i.e., model depth, height, width, and input channel divided by four because four channels share the same pruning structure assuming $g_N = g_M = 4$). CWS leverages both model and pruning information, resulting in more compact storage than traditional CSR.  
% For each four non-zero element in the weights (As continuous four kernel in a filter which are exactly same) we use a Int value (four bytes) to store depth, height, width, channel information, e.g. the first four value - 0, 0, 2, 0 mean the first weight (1) which belongs to the first filter, first channel, depth is 0, height is 0 and width is 2. This format make HWR becomes flexible. Also, it save more space compared with the traditional compact storage - CSR at least four times. 

\begin{figure}[hptb]
  \centering
    \includegraphics[width=0.45\textwidth]{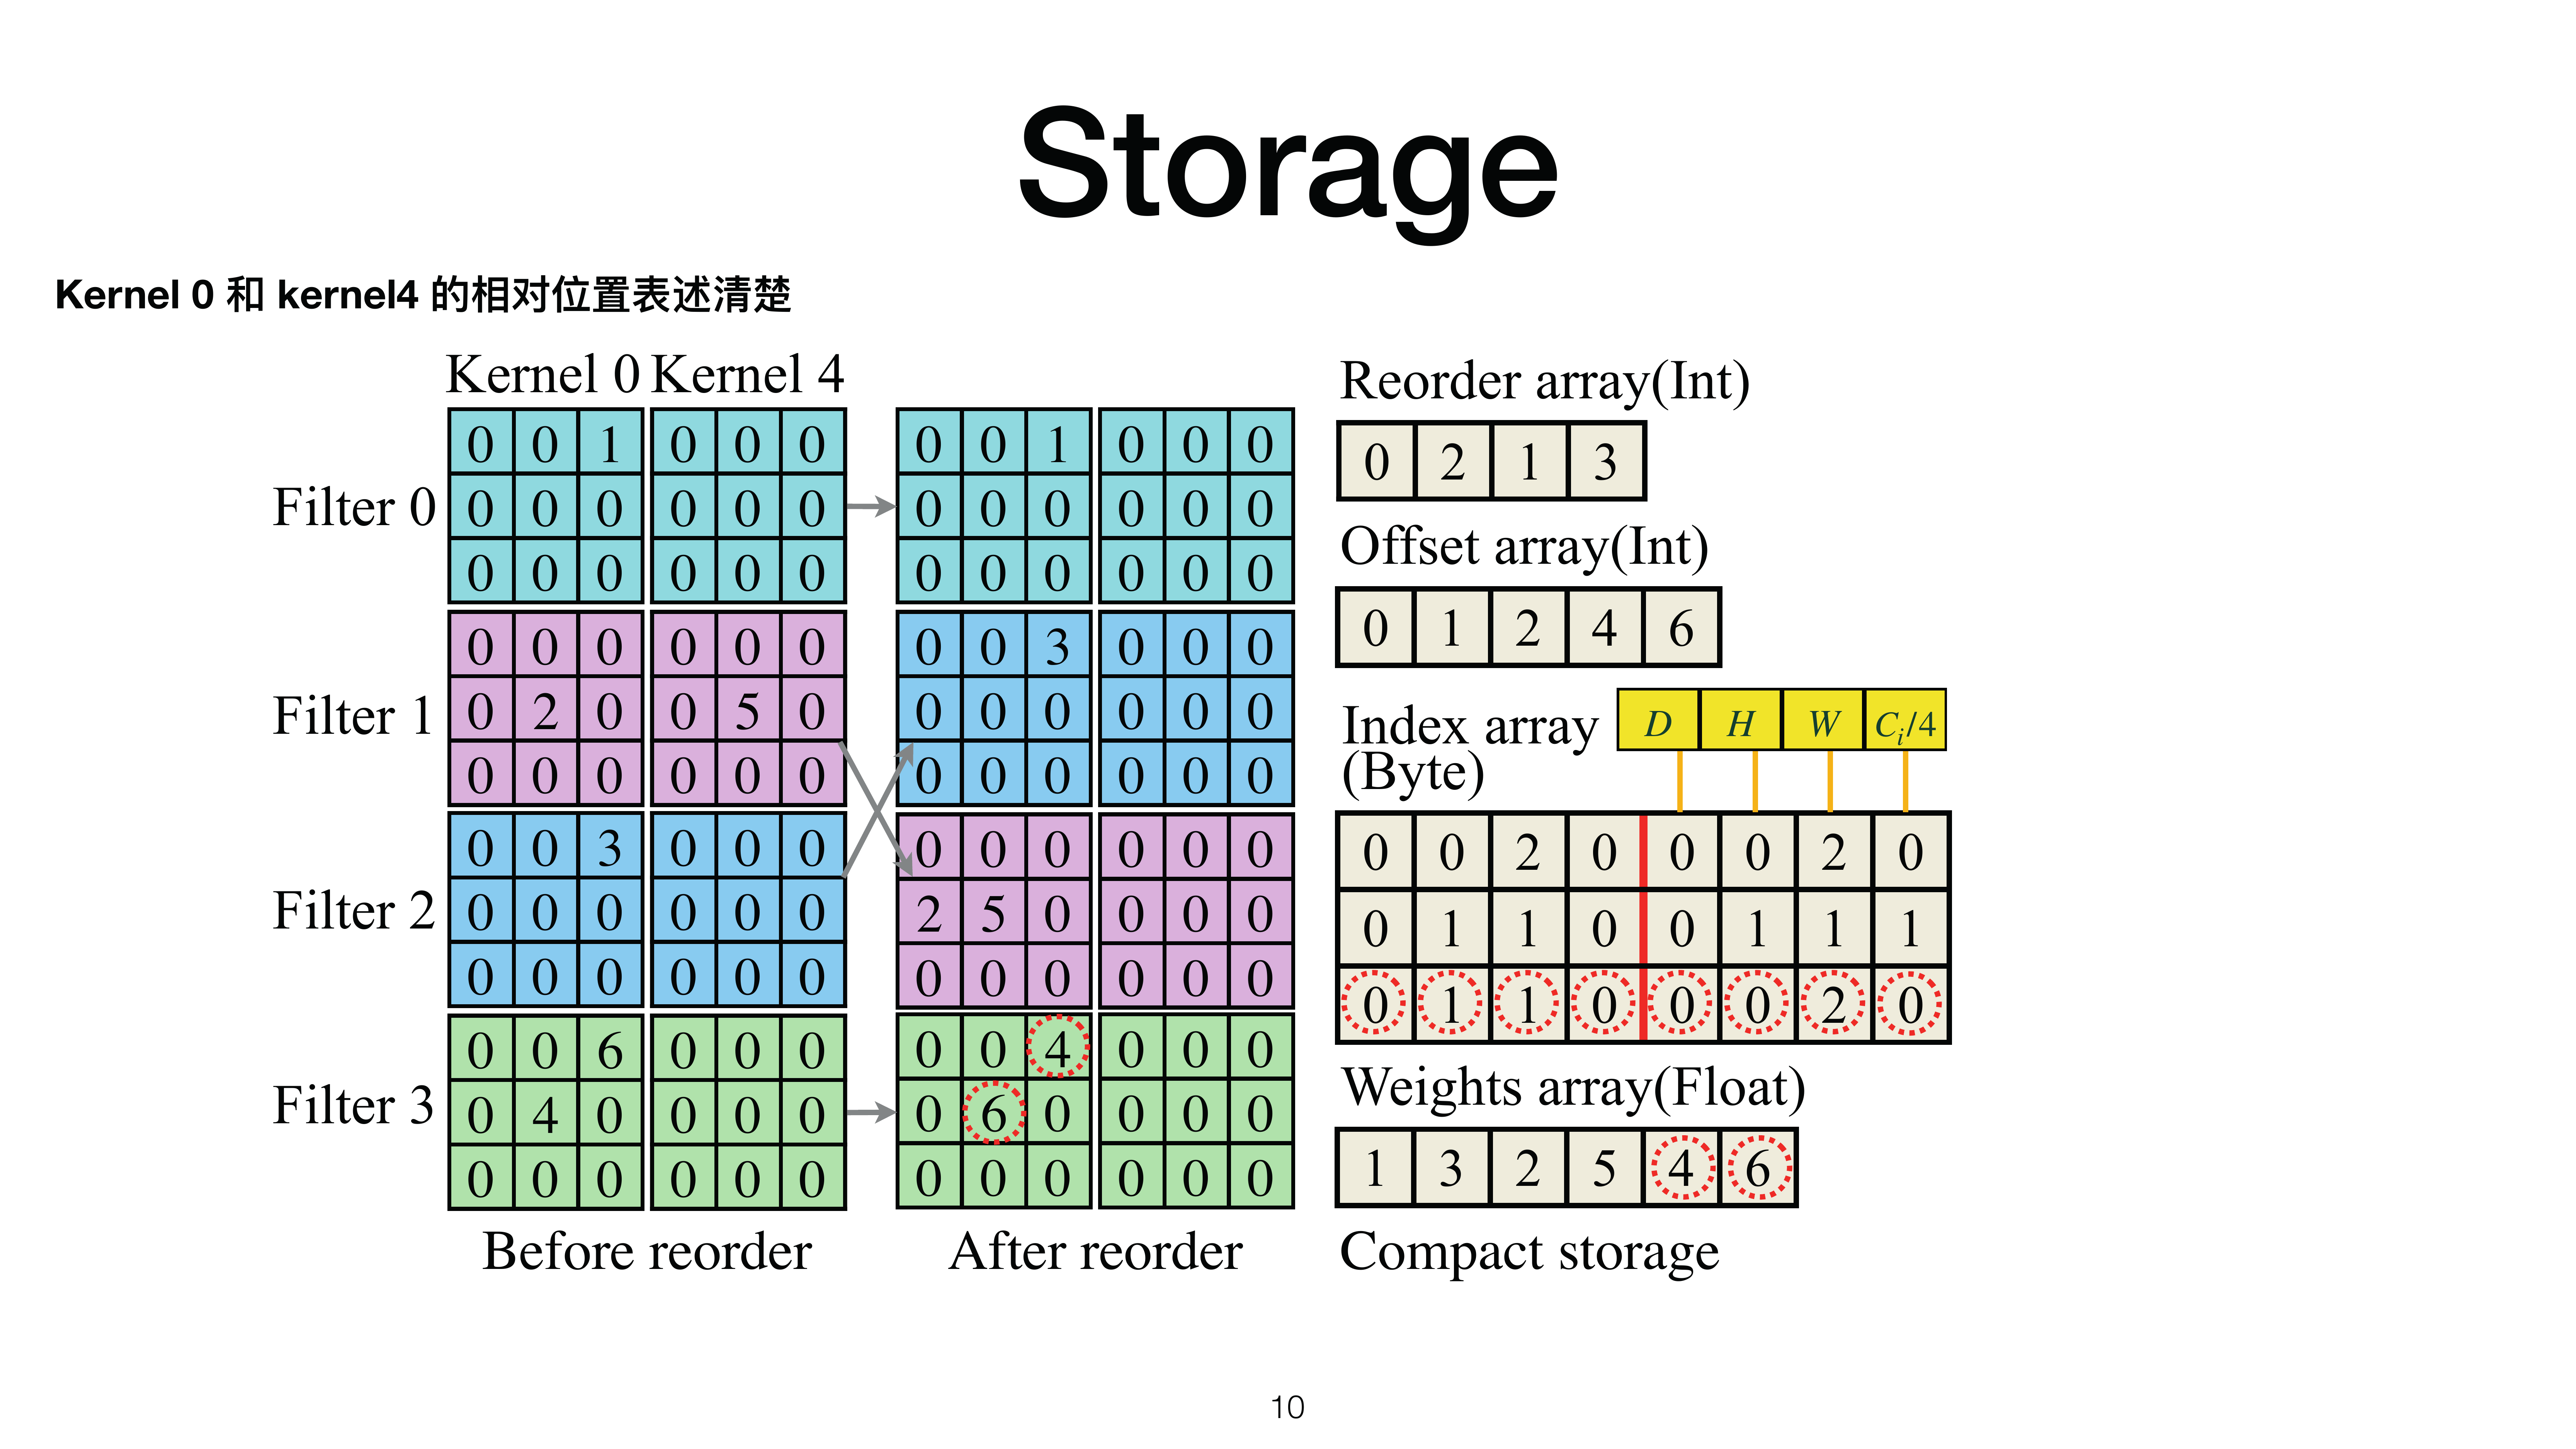}
    \caption{Compact weight storage.}
    \label{fig:compact_storage}
\end{figure}

\paragraph{Loop scheduling.} Based on HWR and CWS, \projectname generates the compressed model execution code. Figure~\ref{fig:loop-schedule} compares the original dense code and \projectname generated compressed code.  In the compressed code, four loops collapse into a single one because the weight index is explicitly stored as an array. \projectname applies loop scheduling on this loop to enable further optimizations (e.g., loop permutation, unrolling, tiling, reorder, etc.).

% \begin{figure*}[hptb]
%   \centering
%   \includegraphics[width=0.98 \textwidth]{figures/inner_loop_scheduling_new.pdf}
%   \caption{{\bf Loop scheduling sample codes generated by compiler for 3D CONV.}}
%   \label{fig:loop-schedule}
% \end{figure*}

\begin{figure}[hptb]
  \centering
    \includegraphics[width=0.45 \textwidth]{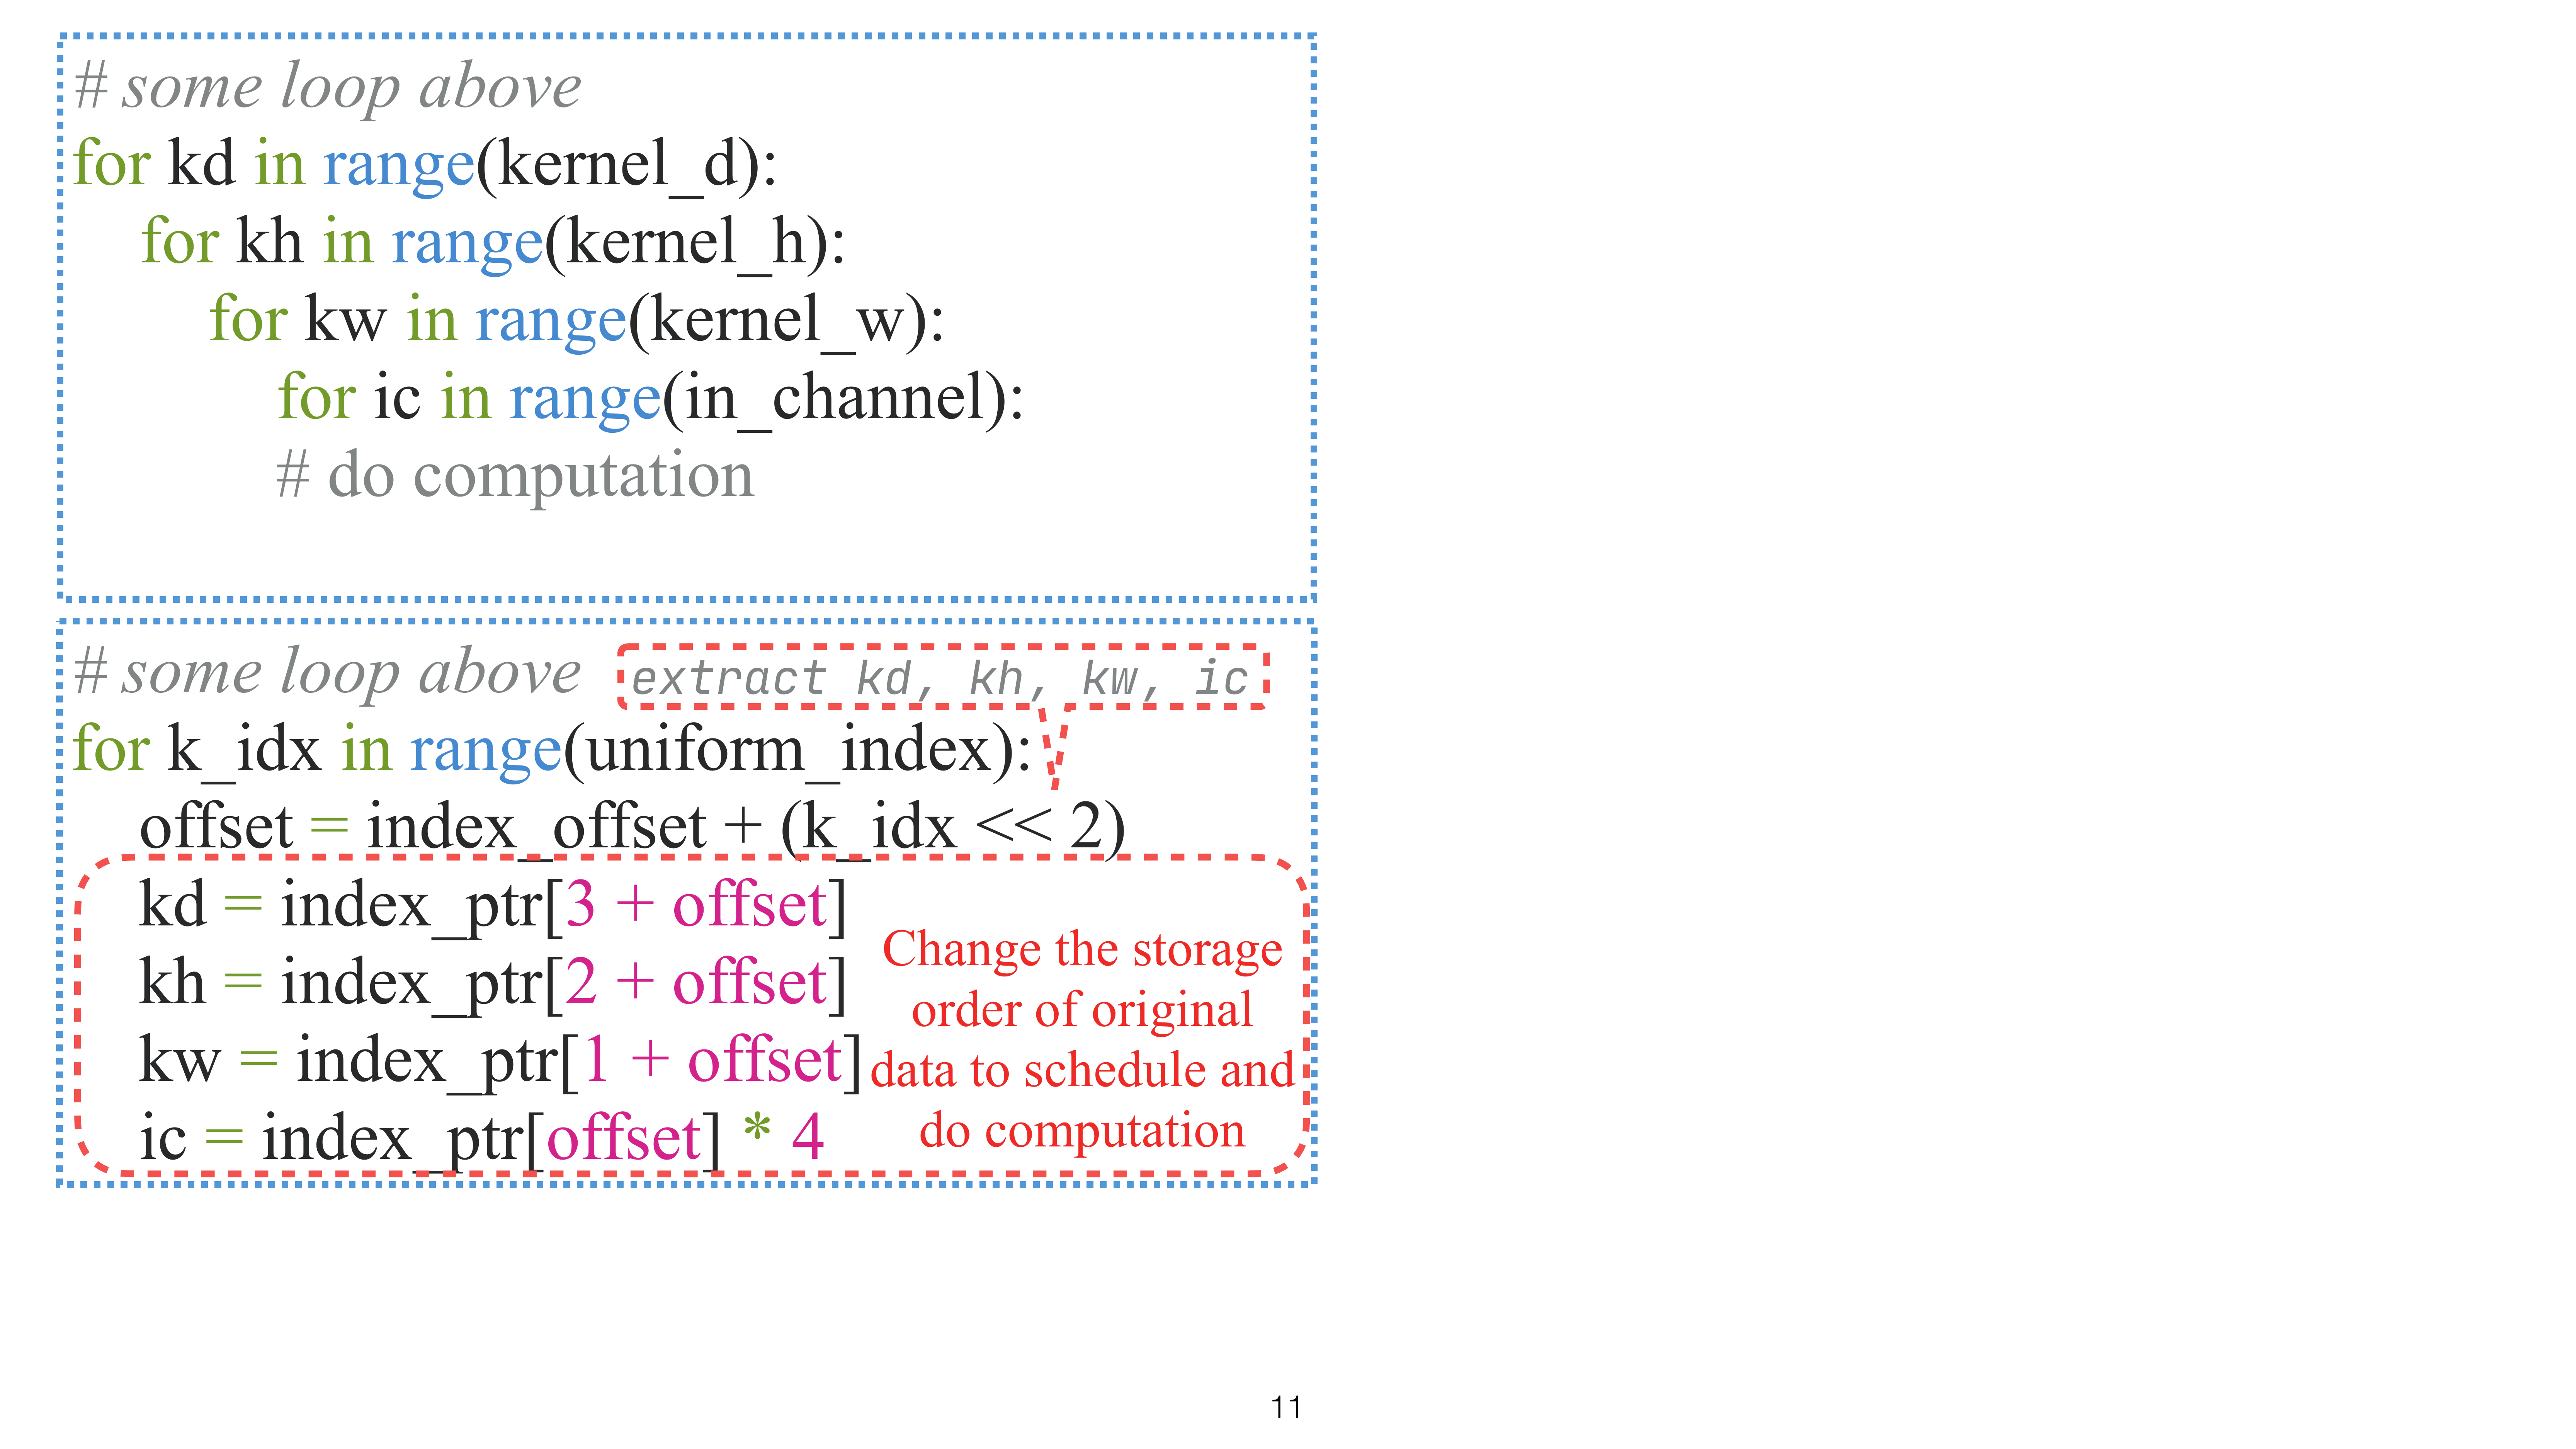}
  \caption{Loop scheduling sample codes generated by compiler for 3D CONV.}
  \label{fig:loop-schedule}
\end{figure}

\paragraph{Other optimizations.}
%tuning, vectorization...
Moreover, \projectname contains an auto-tuning phase to search for the optimal execution configurations such as tiling size, unrolling factor, permutation order, vectorization, code generation, etc. %\todo{more}

%\clearpage
\section{Mobile Acceleration -- Performance and Analysis}\label{sec:appendix-extra-eval}

\subsection{Mobile Acceleration Results on HMDB51 Dataset}

Table~\ref{tab:appendix_performance_report} shows the inference latency comparison of \projectname, MNN, and PyTorch on both mobile CPU and GPU on another dataset, HMDB51. This result is consistent with the result on UCF101 (as shown in Table ~\ref{tab:performance-report}) with the same pruning configuration. Comparing to the mobile CPU version of PyTorch, the fully optimized \projectname (Sparse) achieves up to $10.8\times$ speedup on mobile CPU (S3D), and $28.9\times$ speedup on mobile GPU (R(2+1)D), respectively.  

% Performance table
\begingroup
\begin{table*}[hptb]
\centering
% \small
\begin{tabular}{|c|c|c|cc|cc|cc|cc|}
     \hline
     Framework & MNN & PyTorch & \multicolumn{4}{c|}{\projectname (Dense)} & \multicolumn{4}{c|}{\projectname (Sparse)} \\ \hline
     Device   & \makecell{CPU \\ (ms)} & \makecell{CPU \\ (ms)} & \makecell{CPU \\ (ms)} & Speedup & \makecell{GPU \\ (ms)} & Speedup & \makecell{CPU \\ (ms)} & Speedup & \makecell{GPU \\ (ms)} & Speedup \\ \hline
     \hline
     C3D      & 951 & 2540 & 905  & 2.8$\times$ & 487 & 5.2$\times$  & \textbf{359} & \textbf{7.1$\times$}  & \textbf{144} & \textbf{17.6$\times$} \\ \hline
     R(2+1)D  & -   & 4101 & 1067 & 3.8$\times$ & 515 & 8.0$\times$  & \textbf{393} & \textbf{10.4$\times$} & \textbf{142} & \textbf{28.9$\times$} \\ \hline
     S3D      & -   & 6609 & 1145 & 5.8$\times$ & 566 & 11.7$\times$ & \textbf{610} & \textbf{10.8$\times$} & \textbf{290} & \textbf{22.8$\times$} \\ \hline
\end{tabular}
\caption{Inference latency comparison of \projectname, MNN, and PyTorch on mobile CPU and GPU on the HMDB51 dataset.
MNN does not support R(2+1)D and S3D yet. For RT3D (Sparse), all models are pruned by reweighted regularization algorithm with KGS sparsity. The pruning rate (in FLOPs) is $3.6\times$ for C3D, $3.2 \times$ for R(2+1)D, and $2.1\times$ for S3D, and the accuracy is $53.7\%$, $68.3\%$, and $64.5\%$, respectively. Speedup is the speedup over PyTorch (the CPU version only). }
\label{tab:appendix_performance_report}
\end{table*}
\endgroup

% Break down optimizations among several methods
\subsection{Performance Analysis}

This section studies the effect of \projectname's compiler-based optimizations and explains the underlying reason why \projectname outperforms other frameworks. 

Figure~\ref{fig:opt-speedup} uses eight layers in C3D (trained on UCF101) as an example to show the effect of hierarchical weight reorder ({\tt O1:RE}), loop scheduling ({\tt O2:RE+SH}), and further auto-tuning ({\tt O3:RE+SH+TUNE}). The {\tt No-Opt} baseline is pruned by reweighted regularization algorithm with KGS sparsity with the pruning rate of 3.6$\times$ and accuracy of 80.2$\%$. However, it is not optimized with any compiler optimizations, and sparse weights are stored in the CSR (Compressed Sparse Row) format. This result shows that the pruning itself cannot bring performance gains although it reduces the model size and computation. This is because pruning introduces irregularity and indirect memory access that do not match with the mobile hardware. The subsequent compiler optimizations can fully release pruning benefits and transform them into almost equal times of performance gains.

\begin{figure}[hptb]
  \centering
    \subfloat[C3D-CPU.]{
        \includegraphics[width=0.22\textwidth]{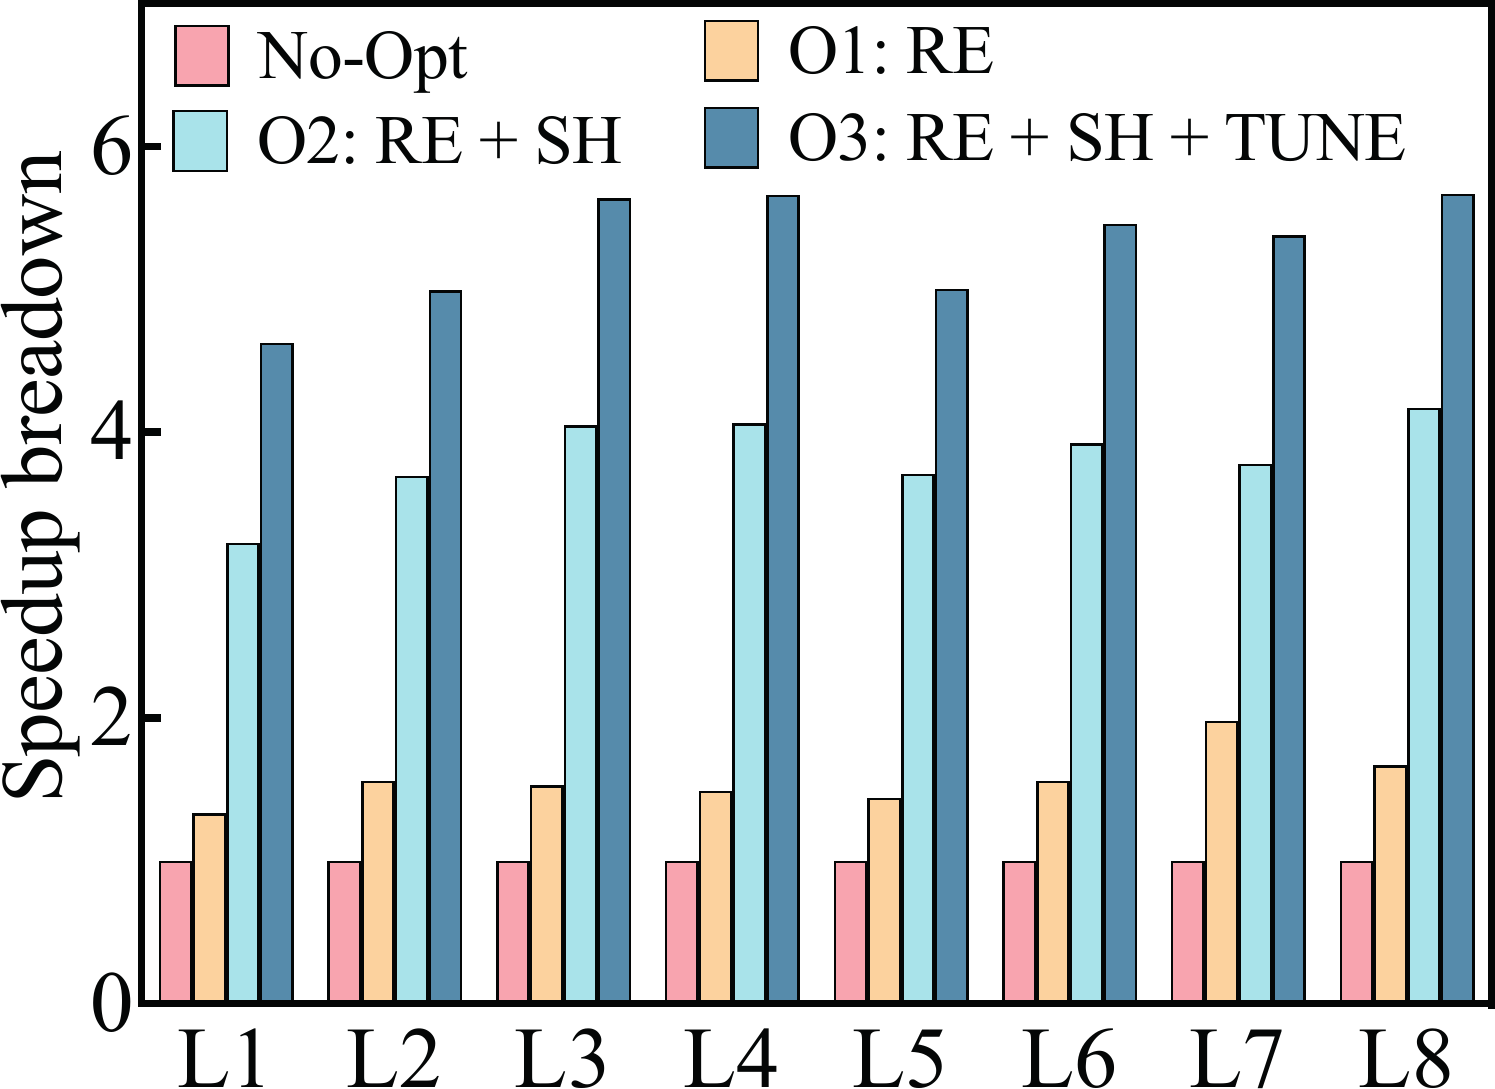}
    }
    \subfloat[C3D-GPU.]{
        \includegraphics[width=0.22\textwidth]{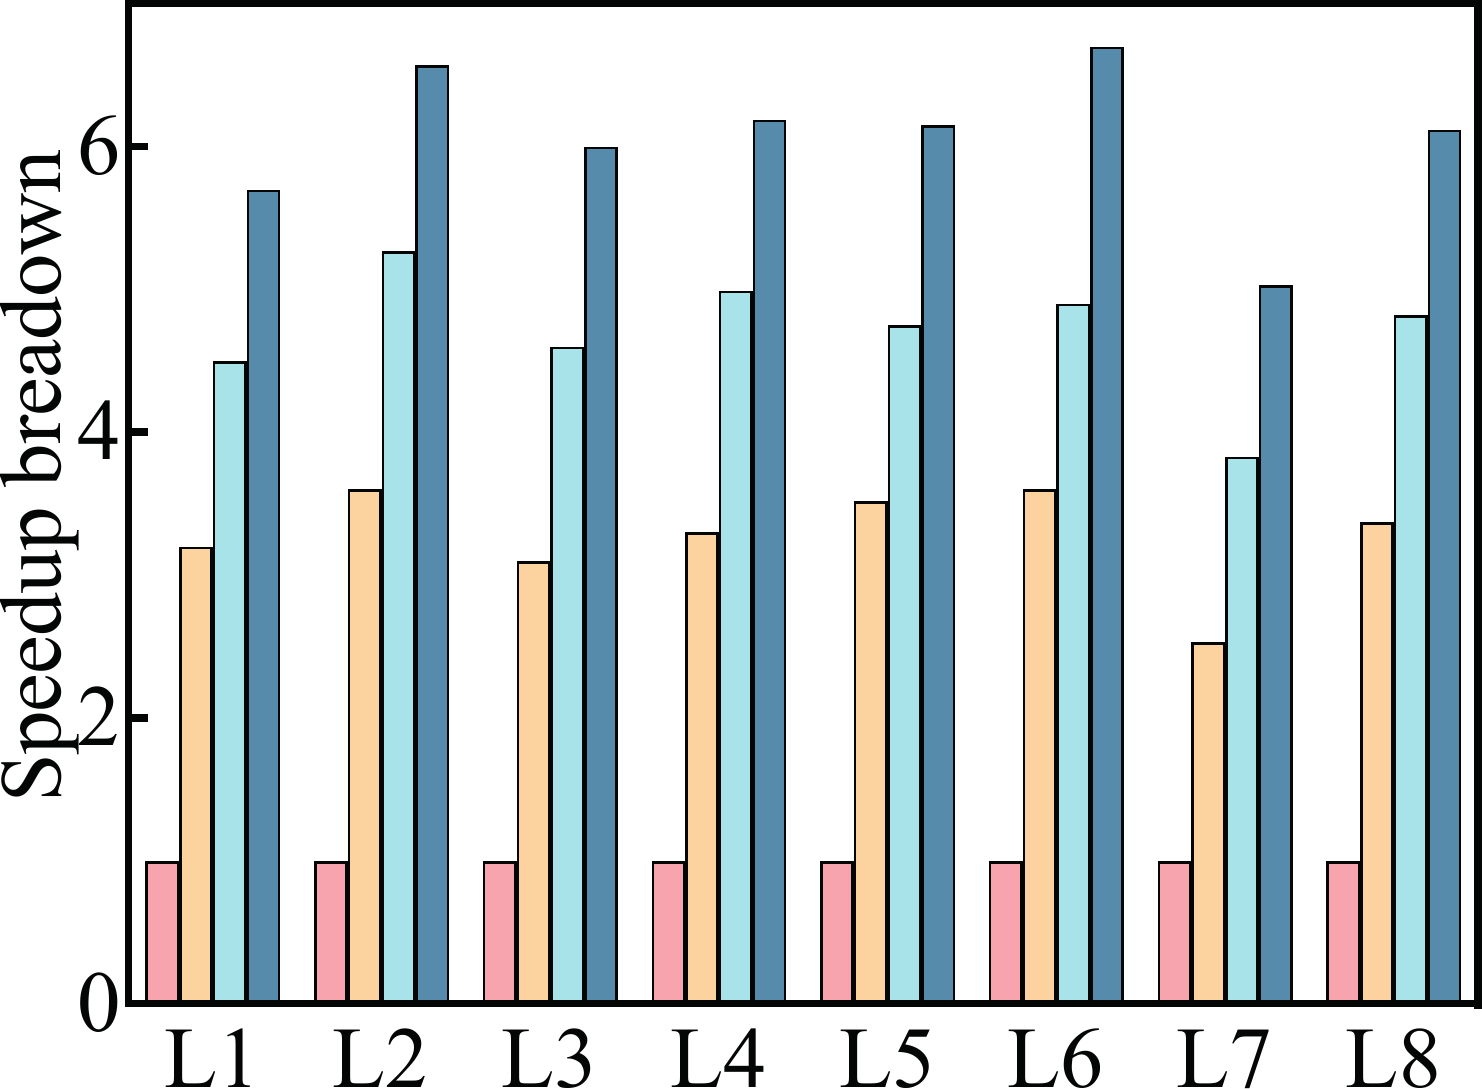}
    }
    \caption{Compiler optimization evaluation on eight unique layers from C3D trained on UCF101. {\tt RE} denotes reorder, {\tt SH} denotes loop scheduling, and {\tt TUNE} denotes auto-tuning.}
    \label{fig:opt-speedup}
\end{figure}

The weight reorder (and associated compact weight storage) ({\tt O1:RE}) can bring 1.3$\times$ to 2.0$\times$ speedup on mobile CPU and 2.5$\times$ to 3.6$\times$ speedup on mobile GPU, respectively. The mobile GPU speedup is higher because mobile GPU prefers the load balance and regular computation brought by weight reorder more than mobile CPU.   To further study the reorder impact, Figure~\ref{fig:reorder-impact} shows the similarity between two neighbor filters (sampled from C3D and R(2+1)D models), demonstrating that the reorder can improve the similarity among continuous filters significantly thus facilitating parallelization.

\begin{figure}[hptb]
  \centering
    \subfloat[C3D.]{
        \raisebox{-\height}{\includegraphics[width=0.22\textwidth]{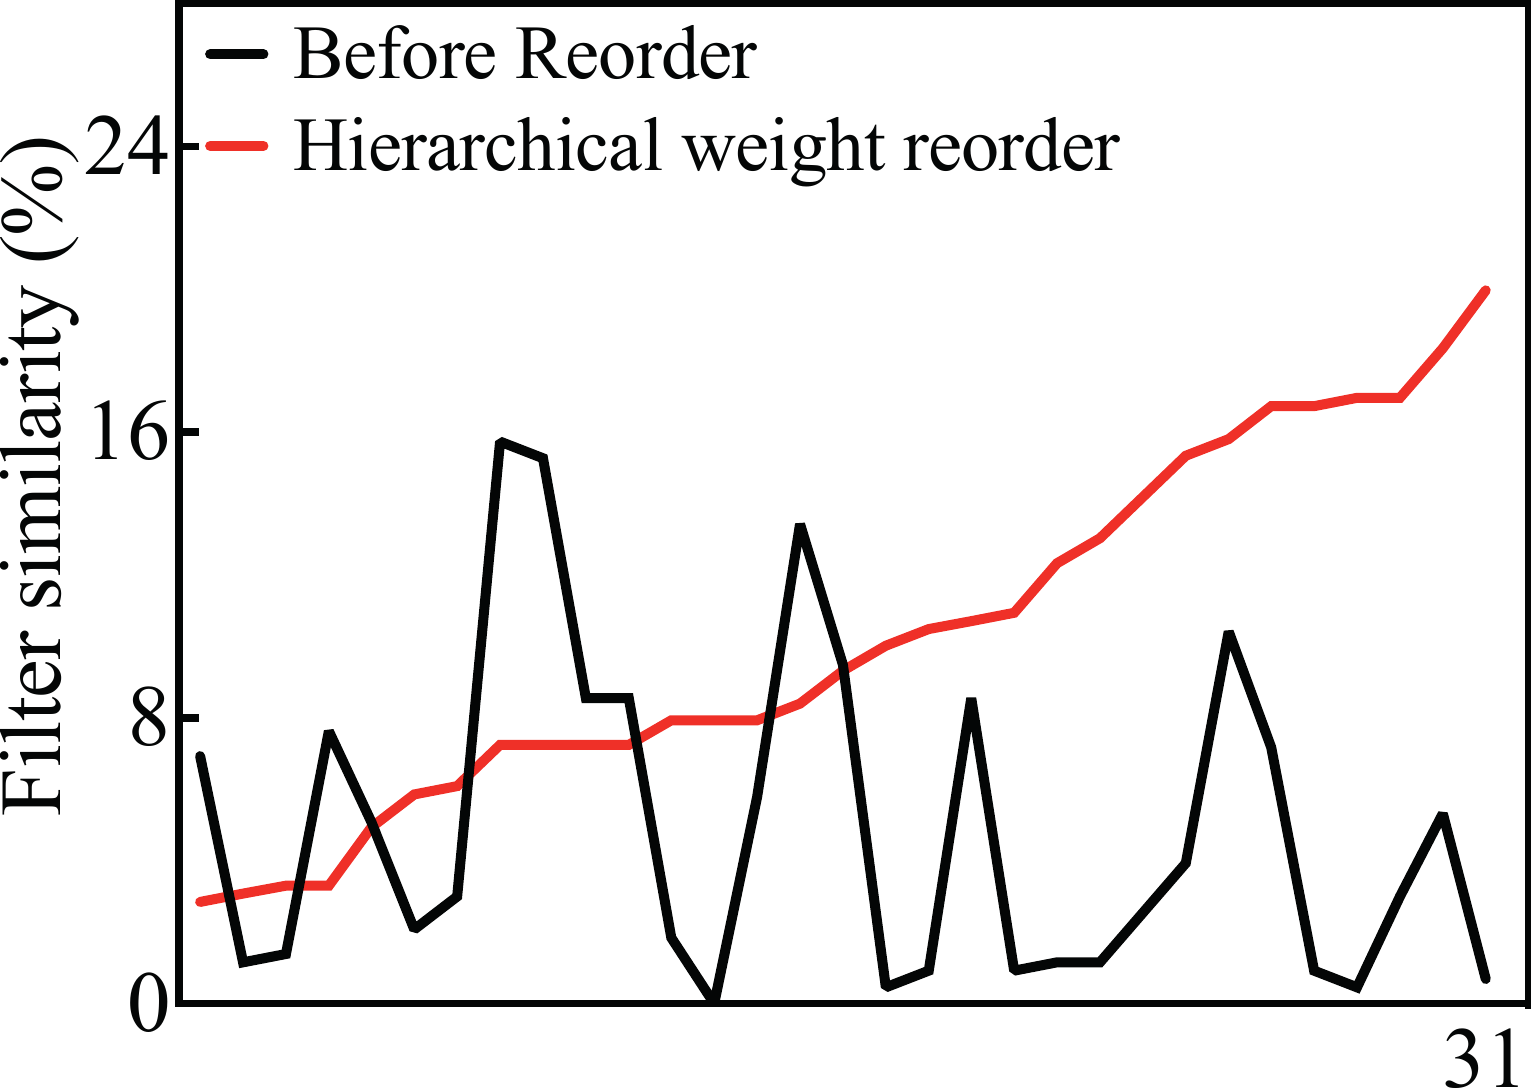}}
    }
    \subfloat[R(2+1)D.]{
        \raisebox{-\height}{\includegraphics[width=0.22\textwidth]{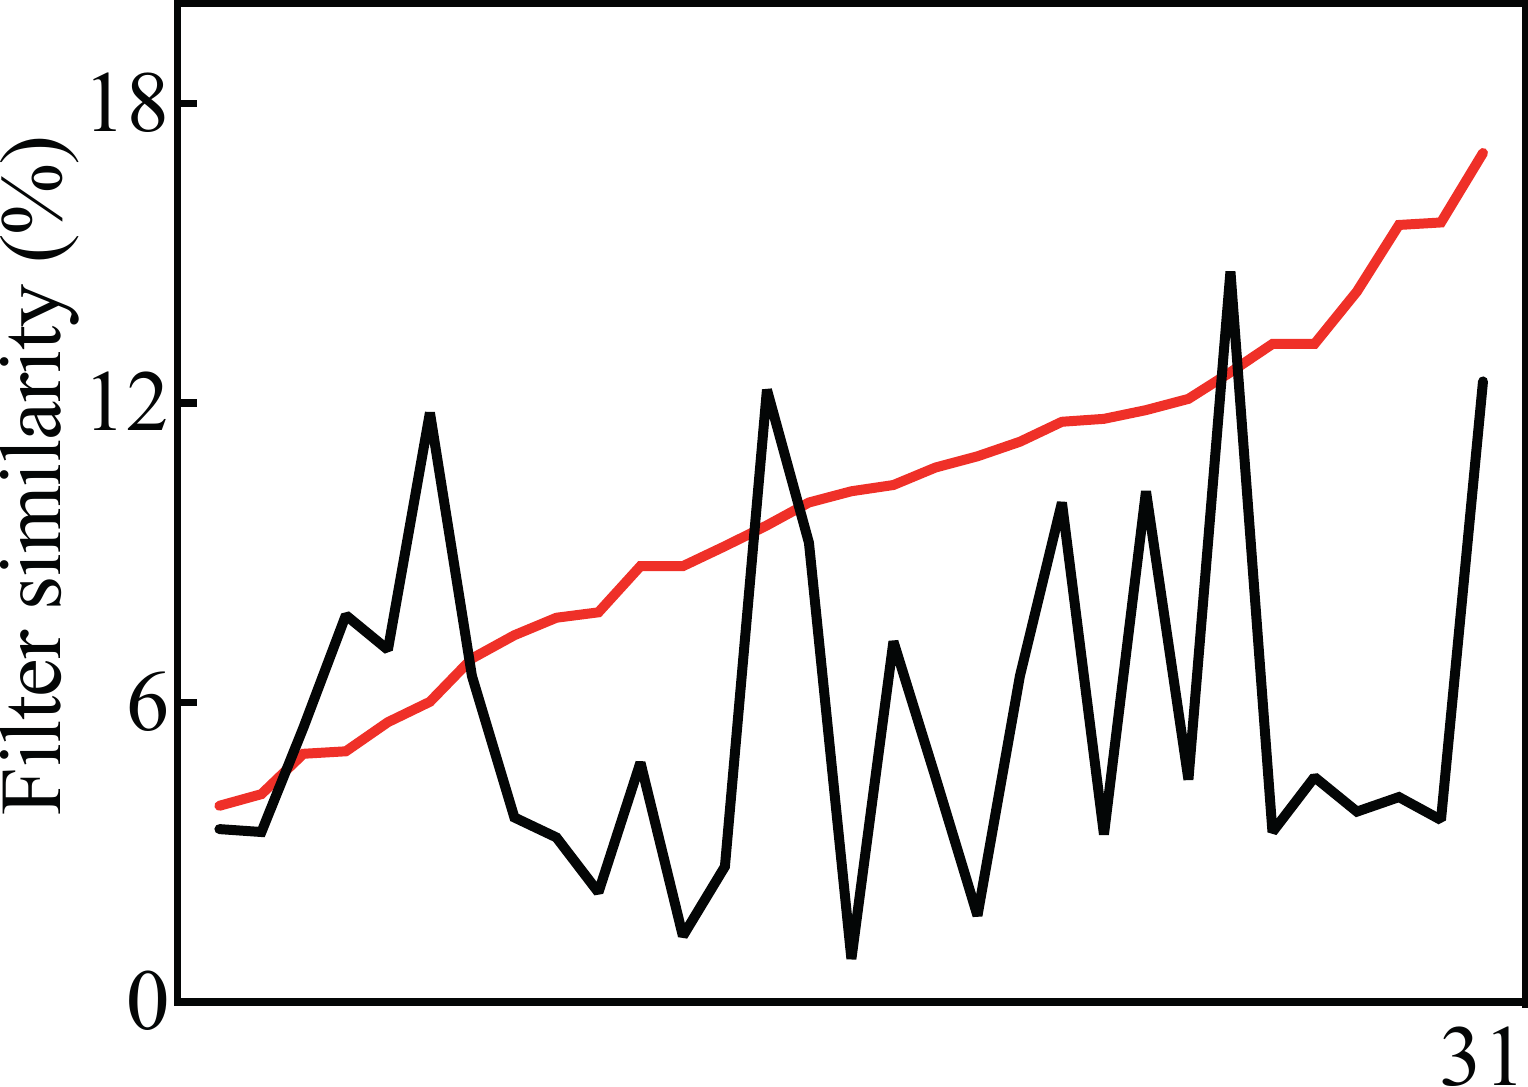}}
    }
    \caption{Hierarchical weight reorder on C3D/R(2+1)D on UCF101. X-axis denotes the first 32 filters with id of 0-31. Y-axis denotes the filter similarity between two neighbor filters.}
    \label{fig:reorder-impact}
\end{figure}

The following loop schedule ({\tt O2:RE+SH}) brings 1.8$\times$ to 2.6$\times$ additional speedup on mobile CPU and 1.2$\times$ to 1.7$\times$ additional speedup on mobile GPU, respectively, and the further auto-tuning ({\tt O3:RE+SH+TUNE}) brings 1.3$\times$ to 1.6$\times$ extra speedup on mobile CPU and 1.2$\times$ to 1.8$\times$ extra speedup on mobile GPU, respectively. Improving data locality is one of the major objectives of these two optimizations. Figure~\ref{fig:cache-miss} (a) compares the cache miss count of each cache layer between PyTorch and \projectname (Sparse). It shows that \projectname (Sparse) has much fewer L1-TLB and L3 (last level) cache misses. Similarly, Figure~\ref{fig:cache-miss} (b) demonstrates the cache miss count reduction brought by different levels of compiler optimizations of \projectname. Because C3D is bounded by memory, this cache miss count result well explains why \projectname outperforms other frameworks like PyTorch.

\begin{figure}[hptb]
  \centering
    \subfloat[\projectname vs. PyTorch.]{
        \raisebox{-\height}{\includegraphics[width=0.22\textwidth]{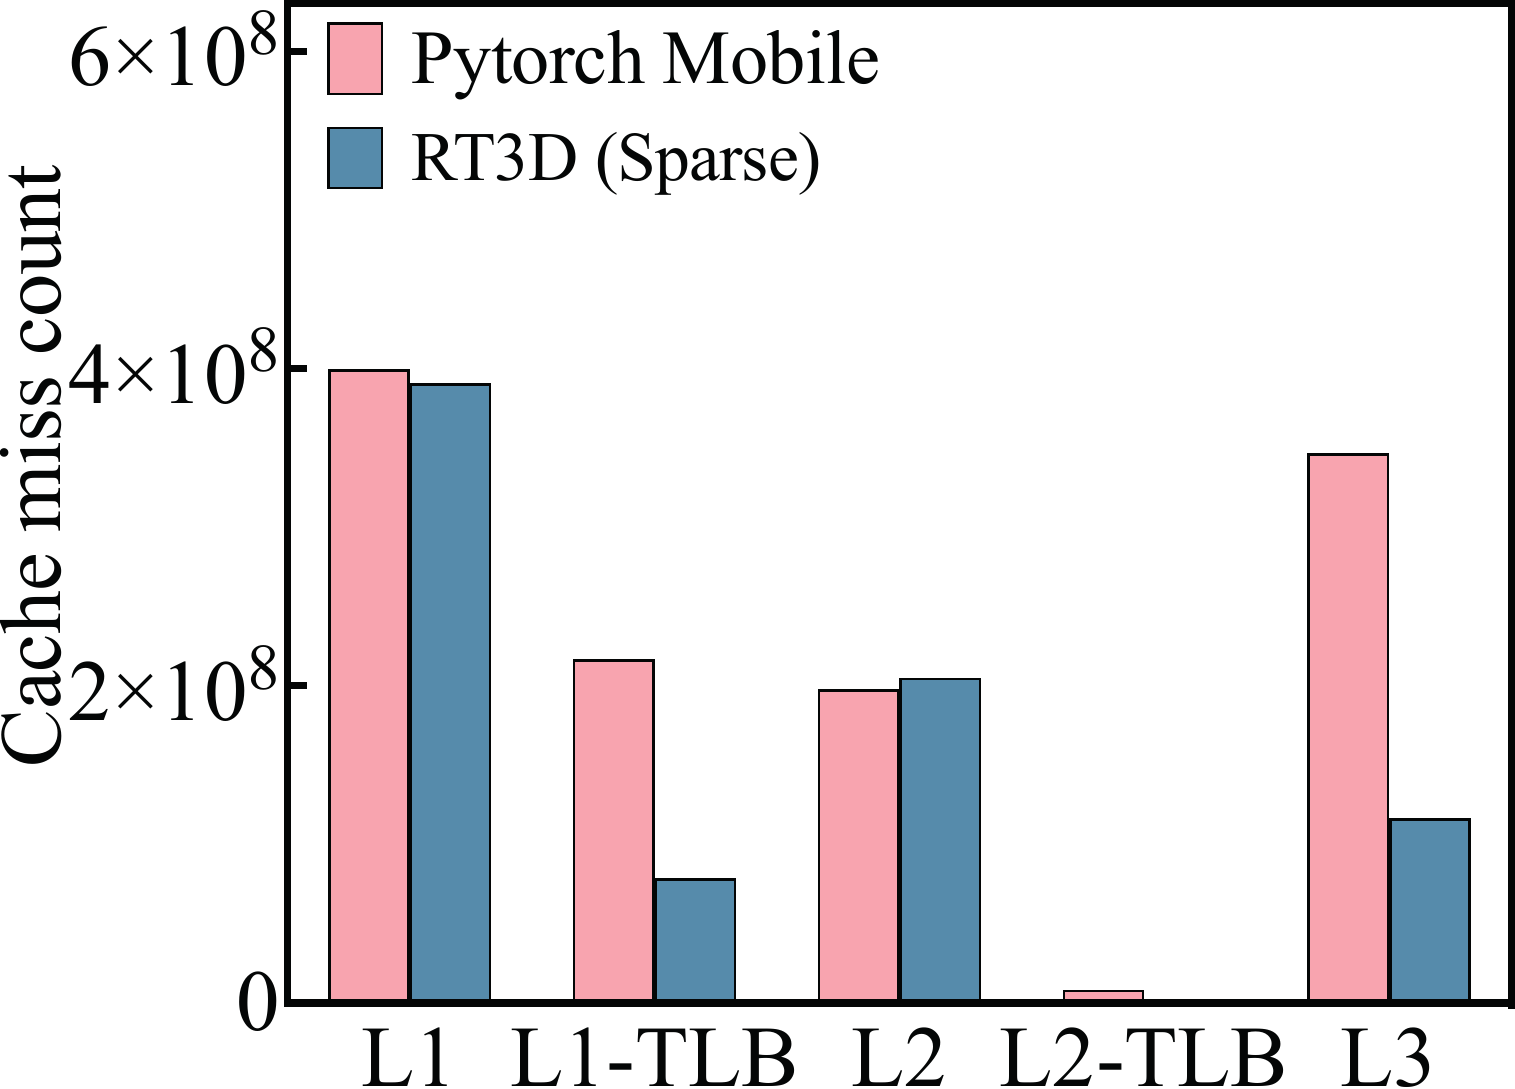}}
    }
    \subfloat[Different levels of Opts.]{
        \raisebox{-\height}{\includegraphics[width=0.22\textwidth]{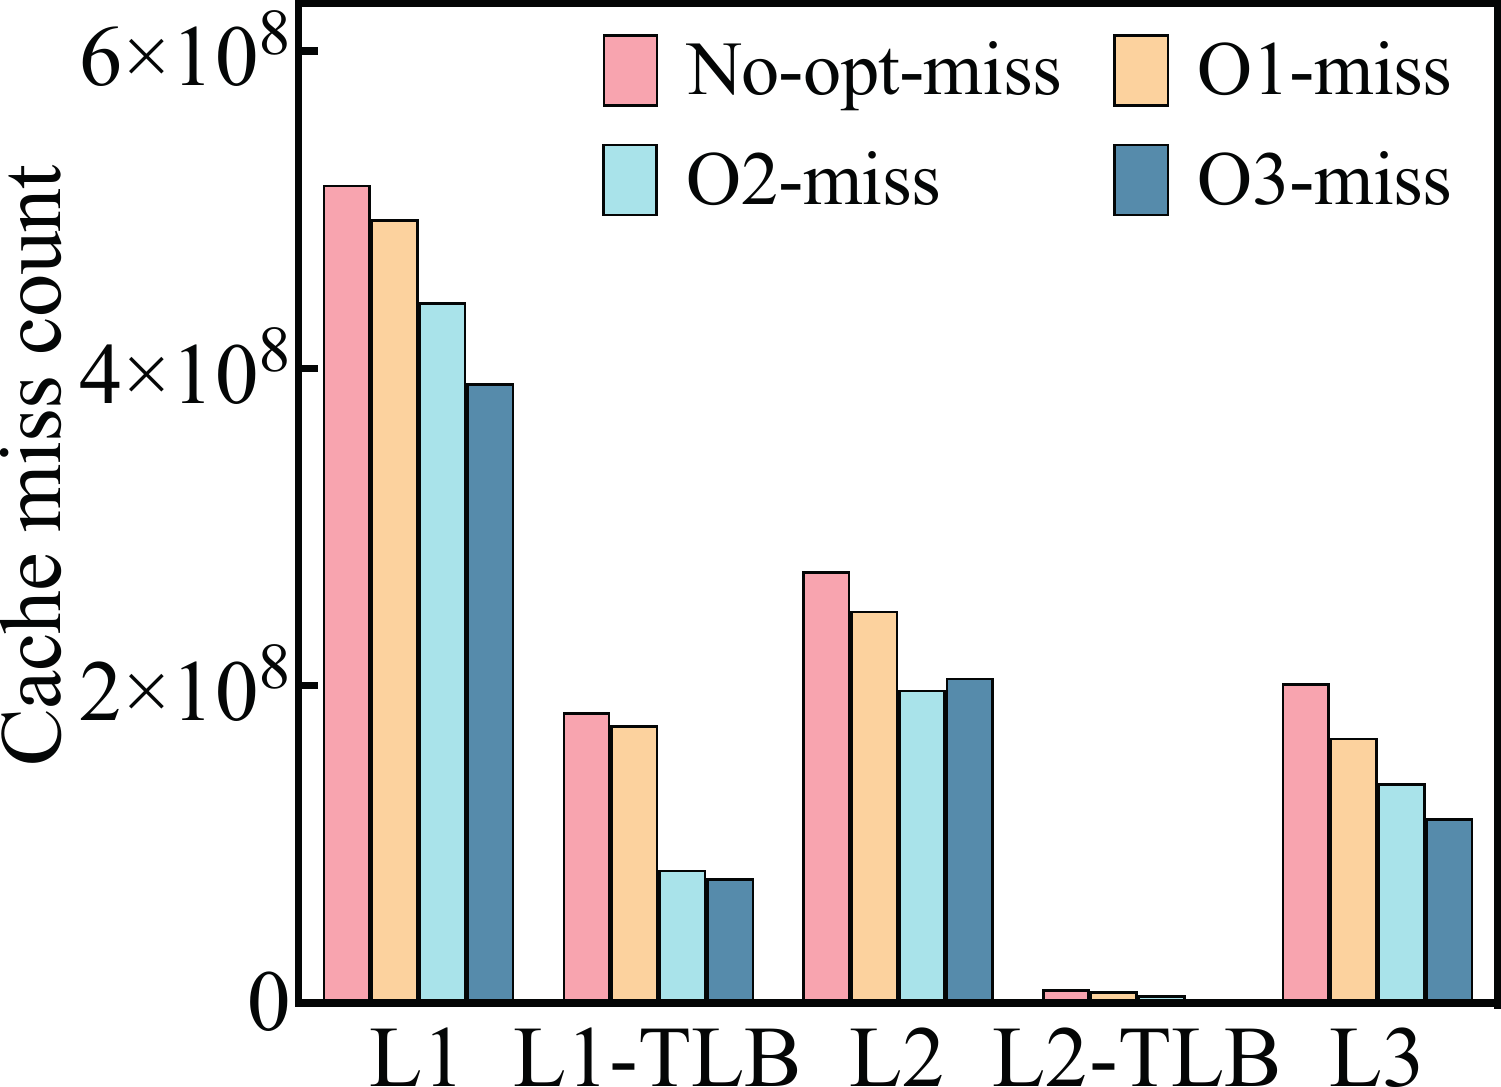}}
    }
    \caption{Cache miss count comparison on L1/L2/L3 data cache and L1/L2 TLB cache with C3D on UCF101.}
    \label{fig:cache-miss}
\end{figure}

% \subsection{Others}
% \begin{itemize}
%     \item Similarity comparison before and after reorder
% \end{itemize}

% % Computation pattern analysis
% \subsection{Computation Pattern Comparison \& Cache Performance Analysis}
% Compare execution time and cache performance:
% \begin{itemize}
%     \item NDHWC with different loop permutation
%     \item NCDHW with different loop permutation
% \end{itemize}

% Model pruning rate vs performance
% \begingroup
% \setlength{\tabcolsep}{2.5pt}
% \renewcommand{\arraystretch}{1.0}
\begin{table*}[hptb]
\centering
% \small
\begin{tabular}{|c|cc|cc|cc|cc|}
    \hline
    \multirow{2}{*}{Model}  & \multicolumn{2}{c|}{MNN} & \multicolumn{2}{c|}{TVM} & \multicolumn{2}{c|}{Tensorflow Lite} & \multicolumn{2}{c|}{Ours (Dense)}\\
                ~           & CPU (ms) & GPU (ms) & CPU (ms) & GPU (ms) & CPU (ms) & GPU (ms) & CPU (ms) & GPU (ms)\\
    \hline \hline
    VGG-16       & 239  & 139  & 251  & 221  & 429  & 307  & \textbf{204}  & \textbf{103} \\ 
    ResNet-18    & 52.4 & 22.5 & 61.5 & 37.6 & 108  & 49.9 & \textbf{41.1} & \textbf{19.8} \\
    MobileNet-V2 & 18.6 & 13.3 & 23.1 & 20.5 & 55.2 & 24.3 & \textbf{17.4} & \textbf{8.7} \\
    \hline

\end{tabular}
\caption{Mobile acceleration comparison with MNN, TVM, and TensorFlow Lite for 2D CNNs. VGG-16, ResNet-18 and MobileNet-V2 on ImageNet dataset are evaluated.}
\label{tab:appendix_2d_cnn}
\end{table*}
% \endgroup

\subsection{Mobile Acceleration Comparison with MNN, TVM and Tensorflow Lite for 2D CNNs}

% Model pruning rate vs performance
% \begingroup
% \setlength{\tabcolsep}{6.5pt} % Default value: 6pt (cell's horizental space)
% \renewcommand{\arraystretch}{1.0} % Default value: 1 (cell's vertical space)
\begin{table*}[hptb]
\centering
% \small
\begin{tabular}{|c|c|c|c|c|c|cc|}
    \hline
    \multirow{2}{*}{Model}  & Sparsity & Base Top-1 & Pruning Top-1 & FLOPs & Pruning Rate & \multicolumn{2}{c|}{Latency (ms)}\\
                            & Scheme   & Accuracy   & Accuracy      & after Pruning & of FLOPs & CPU & GPU\\
    \hline \hline
    % C3D results
    \multirow{2}{*}{C3D}    & Vanilla & \multirow{2}{*}{53.5\%} & \multirow{2}{*}{53.5\%} & 18.4G & 2.1$\times$ & 573 & 254 \\
                            & \textbf{KGS} & ~ & ~ & \textbf{9.7G}  & \textbf{4.0$\times$} & \textbf{330} & \textbf{136} \\ \hline\hline
    % R2+1D results
    \multirow{2}{*}{R(2+1)D} & Vanilla & \multirow{2}{*}{71.3\%} & \multirow{2}{*}{68.5\%} & 18.5G & 2.2$\times$& 578 & 248 \\
                             & \textbf{KGS} & ~ & ~ & \textbf{13.6G} & \textbf{3.0$\times$}& \textbf{460} & \textbf{175} \\ \hline
\end{tabular}
\caption{Comparison between Vanilla and KGS sparsity schemes: pruning rate, and inference latency with the same pruning Top-1 accuracy on the HMDB51 dataset. Reweighted regularization pruning is applied for all models.}
\label{tab:appendix_prune_ablation}
\end{table*}
% \endgroup

To demonstrate the generality and the superiority of our baseline \projectname (Dense), Table~\ref{tab:appendix_2d_cnn} compares both the mobile CPU and GPU inference latency of \projectname (Dense), MNN, TVM, and TensorFlow Lite with representative 2D CNNs, VGG-16, ResNet-18, and MobileNet-V2 on ImageNet dataset. \projectname clearly outperforms all other frameworks for all 2D CNNs.

\subsection{Ablation Study}

Table~\ref{tab:appendix_prune_ablation} compares two sparsity schemes, Vanilla and KGS in terms of pruning rate and inference latency by controlling the same pruning top-1 accuracy on another dataset HMDB51, and gets consistent results with Table~\ref{tab:prune_ablation} that is on UCF101.

\subsection{Portability Evaluation}
\projectname is also tested on two other phones to validate its portability (as shown in Figure~\ref{fig:portibility}).
 We take C3D as an example because other models show the same trend. Only \projectname supports mobile GPUs.
  %\projectname's design and optimization are general to any other brand or type of mobile device. 
\projectname gains the similar performance speedup over other frameworks on all platforms. In particular, \projectname shows more stable performance on the older generation of mobile devices. This is because our pruning (and associated compiler optimization) significantly reduces the overall computation and memory requirement, thus tolerating a more resource-constrained environment.
Thus, we claim \projectname has the potential to run 3D CNN on many mobile devices (even weaker ones like Raspberry Pi) in real-time.

\begin{figure}[hptb]
  \centering
    \subfloat[Snapdragon 855.]{
        \raisebox{-\height}{\includegraphics[width=0.22\textwidth]{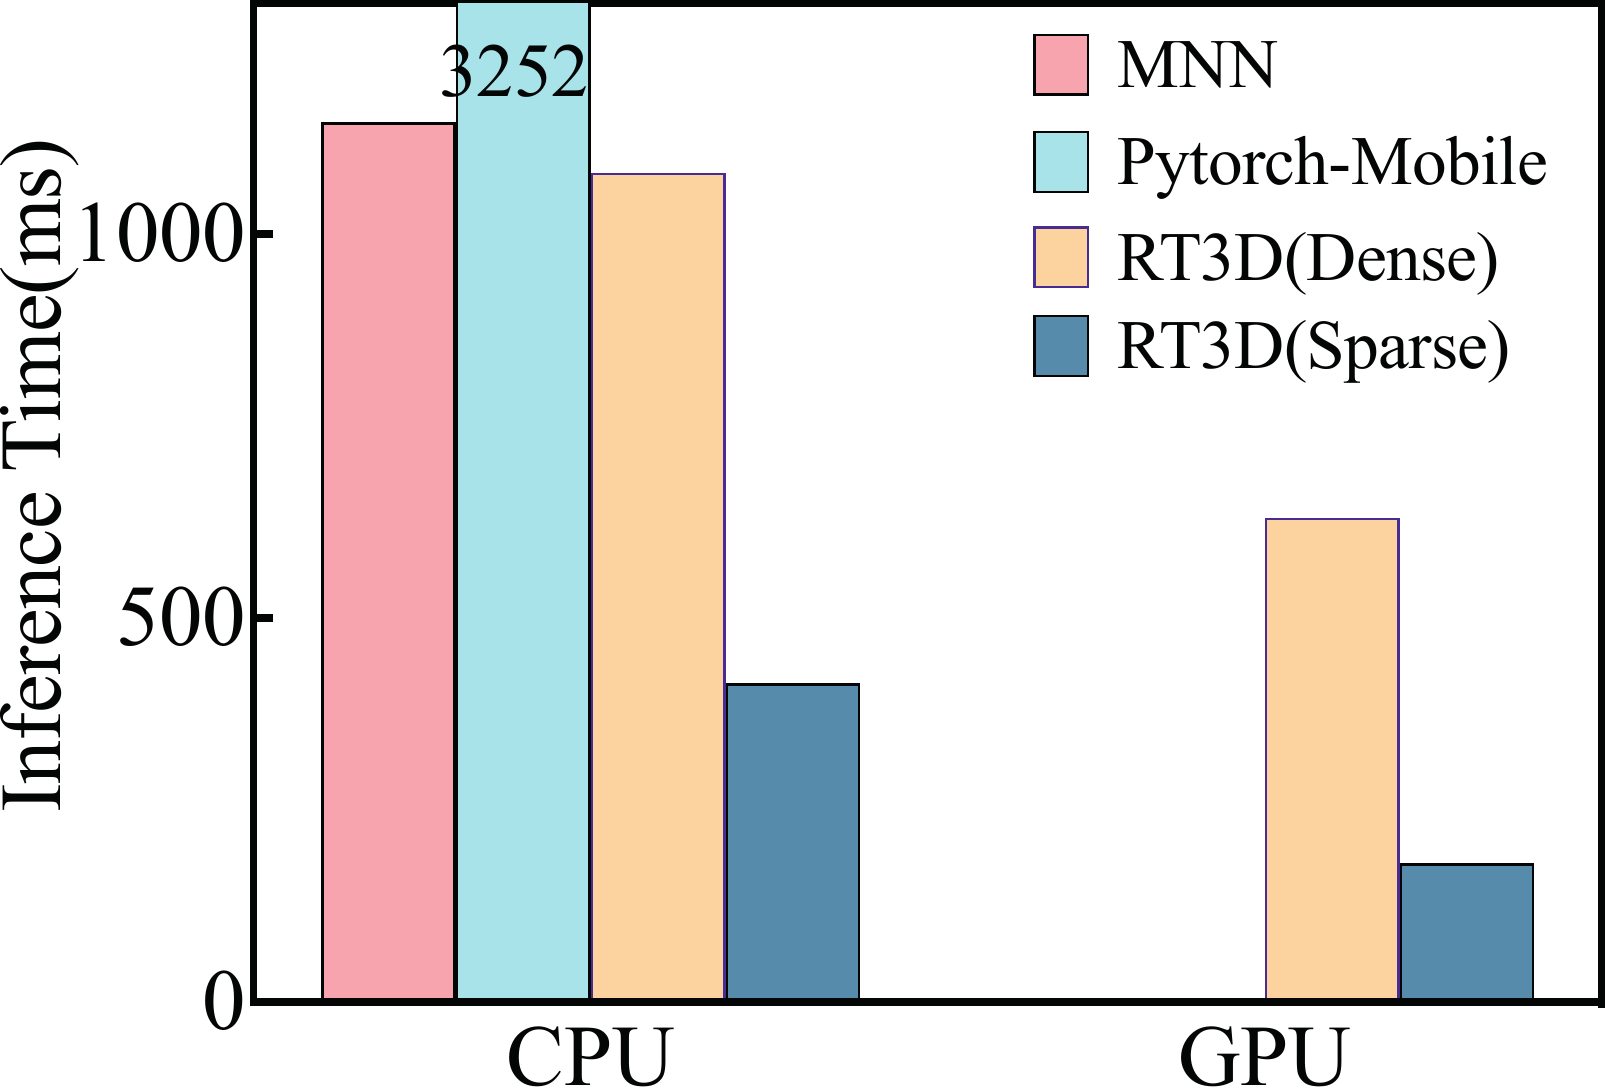}}
    }
    \subfloat[Kirin 980.]{
        \raisebox{-\height}{\includegraphics[width=0.22\textwidth]{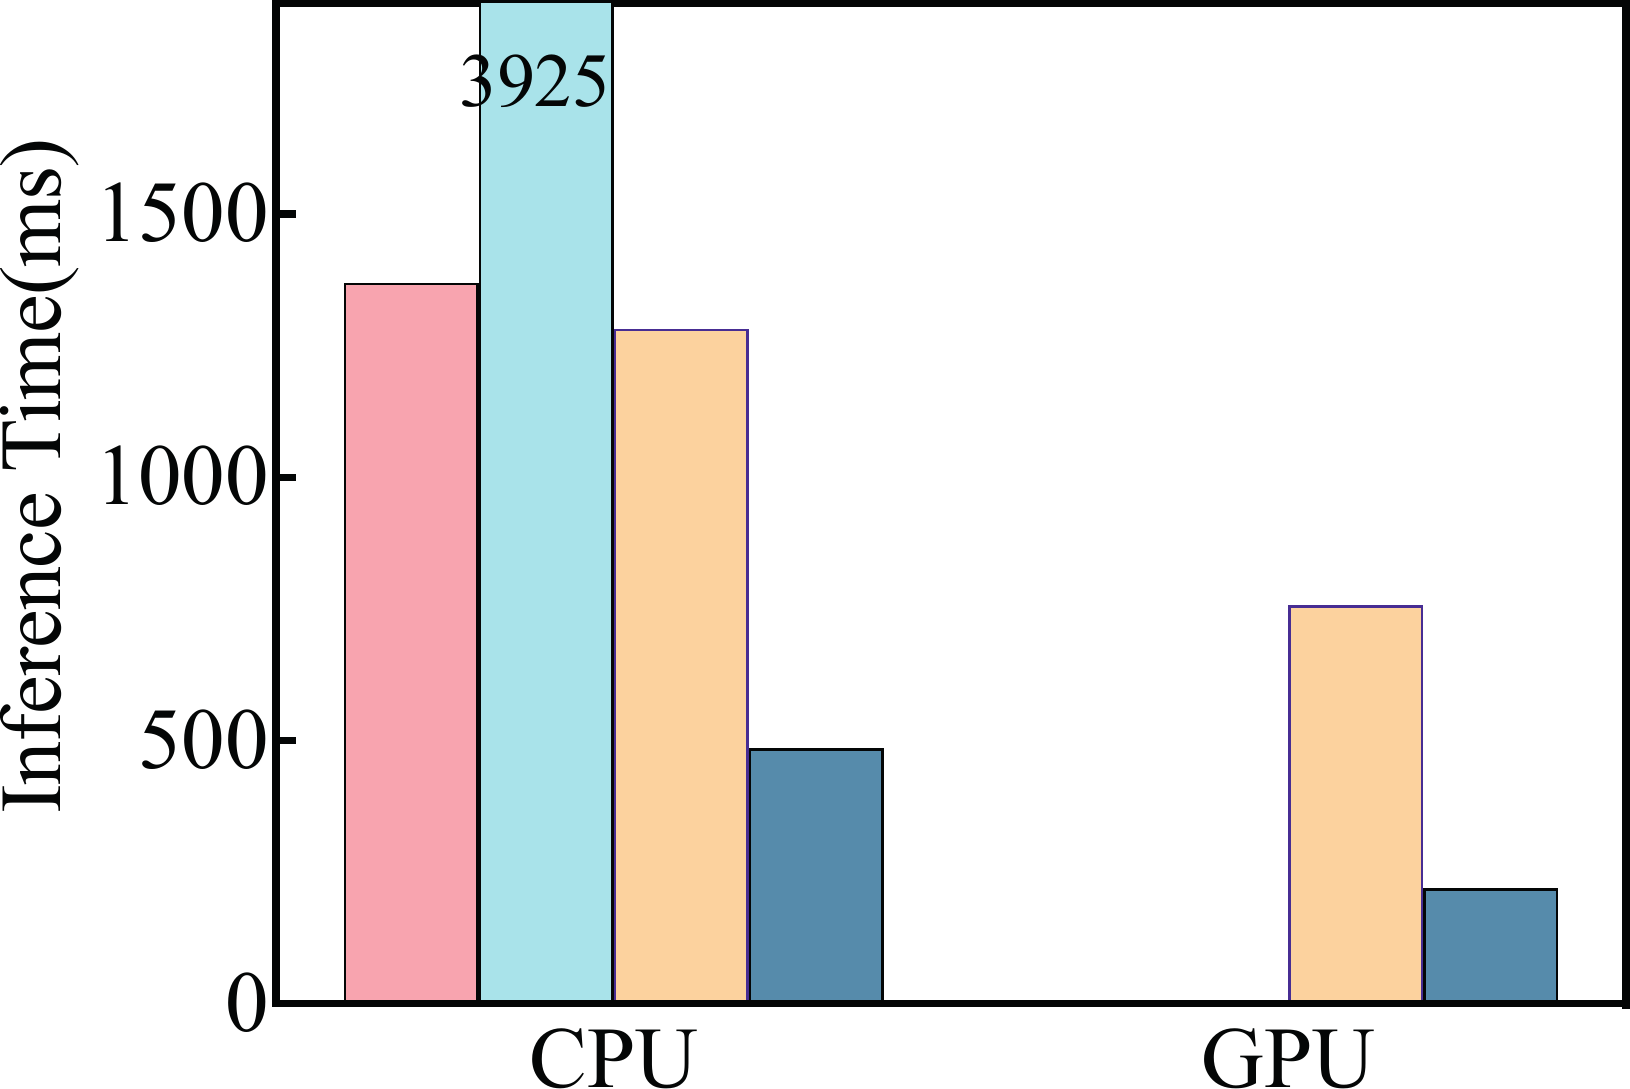}}
    }
    \caption{Portability evaluation with C3D with UCF101 on Snapdragon 855 and Kirin 980. Only \projectname supports mobile GPU execution.}
    \label{fig:portibility}
\end{figure}
%\textcolor{red}{Mention demo video uploaded in the supplementary material if available.}
%\textcolor{red}{No more ADMM.}
